# Supplementary material for: Boosting One-Point Derivative-Free Online Optimization via Residual Feedback
Source: arXiv:2010.07378 source file (2020-12-03)
Supplement: Supplementary file 1 [file appendix.tex]

\newpage
\onecolumn
\appendix
\noindent {\Large \textbf{Supplementary Materials}}
\section{Zeroth-Order Policy Optimization for A Large-Scale Multi-Stage Decision Making Problem}
In this section, we consider a large-scale multi-stage resource allocation problem. Specifically, we consider $16$ agents that are located on a $4 \times 4$ grid. At agent $i$, resources are stored in the amount of $m_i(k)$ and there is also a demand for resources in the amount of $d_i(k)$ at instant $k$.
In the meantime, agent $i$ also decides what fraction of resources $a_{ij}(k) \in [0, 1]$ it sends to its neighbors $j \in  \mathcal{N}_i$ on the grid. The local amount of resources and demands at agent $i$ evolve as $m_i(k+1) = m_i(k) - \sum_{j \in \mathcal{N}_i} a_{ij}(k) m_i(k) + \sum_{j \in \mathcal{N}_i} a_{ji}(k) m_j(k) - d_i(k)$ and $d_i(k) = A_i \sin(\omega_i k + \phi_i) + w_{i,k}$,
where $w_{i,k}$ is the noise in the demand. At time $k$, agent $i$ receives a local reward $r_i(k)$, such that $r_i(k) = 0$ when $m_i(k) \geq 0$ and $r_i(k) = -m_i(k)^2$ when $m_i(k) < 0$. Let agent $i$ makes its decisions according to a parameterized policy function $\pi_{i, \theta_i}(o_i): \mathcal{O}_i \rightarrow [0,1]^{|\mathcal{N}_i|}$, where $\theta_i$ is the parameter of the policy function $\pi_i$, $o_i \in \mathcal{O}_i$ denotes agent $i$'s observation, and $|\mathcal{N}_i|$ represents the number of agent $i$'s neighbors on the grid. 

Our goal is to train a policy that can be executed in a fully distributed way based on agents' local information. Specifically, during the execution of policy functions $\{\pi_{i, \theta_i}(o_i)\}$, we let each agent only observe its local amount of resource $m_i(k)$ and demand and $d_i(k)$, i.e., $o_i(k) = [m_i(k), d_i(k)]^T$.
In addition, the policy function $\pi_{i, \theta_i}(o_i)$ is parameterized as the following: $a_{ij} = \exp(z_{ij}) / \sum_{j}\exp(z_{ij})$, where $z_{ij} = \sum_{p = 1}^{9} \psi_p(o_i) \theta_{ij}(p)$ and $\theta_i = [\dots, \theta_{ij}, \dots]^T$. Specifically, the feature function $\psi_p(o_i)$ is selected as $\psi_p(o_i) = \|o_i - c_p\|^2$, where $c_p$ is the parameter of the $p$-th feature function. The goal for the agents is to find an optimal policy $\pi^\ast = \{\pi_{i, \theta_i}(o_i)\}$ so that the global accumulated reward
\begin{align}
	\label{eqn:Obj}
	J(\theta) = \sum_{i=1}^{16} \sum_{k = 0}^{K} \gamma^{k} r_i(k) 
\end{align} 
is maximized, where $\theta = [\dots, \theta_i, \dots]$ is the global policy parameter, $K$ is the horizon of the problem, and $\gamma$ is the discount factor. Effectively, the agents need to make decisions on $64$ actions, and each action is decided by $9$ parameters. Therefore, the problem dimension is $d = 576$.
To implement zeroth-order policy gradient estimators \eqref{eqn:OnePoint} and \eqref{eqn:GradientEstimate_Noise} to find the optimal policy, at iteration $t$, we let all agents implement the policy with parameter $\theta_t + \delta u_t$, collect rewards $\{r_i(k)\}$ at  time instants $k = 0, 1, \dots, K$ and compute the noisy policy value according to~\eqref{eqn:Obj}. Then, the zeroth-order policy gradient is estimated using~\eqref{eqn:OnePoint} or \eqref{eqn:GradientEstimate_Noise}. On the contrary, when the two-point zeroth-order policy gradient estimator~\eqref{eqn:TwoPoint} is used, at each iteration $k$, all agents need to evaluate two policies $\theta_t \pm \delta u_t$ to update the policy parameter once. In Figure~\ref{fig:resource}, we present the performance of using zeroth-order policy gradients~\eqref{eqn:OnePoint}, \eqref{eqn:TwoPoint} and \eqref{eqn:GradientEstimate_Noise} to solve this large-scale multi-stage resource allocation problem, where the discount factor is set as $\gamma = 0.75$ and the length of horizon $K = 30$. Each algorithm is run for $10$ trials. 
We observe that policy optimization with the proposed residual-feedback gradient estimate~\eqref{eqn:GradientEstimate_Noise} improves the optimal policy parameters with the same learning rate as the two-point zeroth-order gradient estimator~\eqref{eqn:TwoPoint}, where the learning rate is measured by the number of episodes the agents take to evaluate the policy parameter iterates.
In the meantime, both estimators perform much better than the one-point policy gradient estimate~\eqref{eqn:OnePoint} considered in \cite{fazel2018global,malik2018derivative}.
\begin{figure}[t]
	\centering
	\includegraphics[width = .7\columnwidth]{Resource_Alloc}
	\caption{\small The convergence rate of applying the proposed residual one-point feedback~\eqref{eqn:GradientEstimate_Noiseless} (blue), the two-point oracle \eqref{eqn:TwoPoint} in \cite{nesterov2017random} (orange) and the one-point oracle~\eqref{eqn:OnePoint} in \cite{flaxman2005online} (green) to the large-scale stochastic multi-stage resource allocation problem. The vertical axis represents the total rewards and the horizontal axis represents the number of episodes the agents take to evaluate their policy parameter iterates during the policy optimization procedure.}
	\label{fig:resource}
\end{figure}

\section{Proof of Lemma~\ref{lem:BoundSecondMoment_Det}}
\label{sec:BoundSecondMoment_Det}
First, we show the bound when $f(x) \in C^{0,0}$. Recalling the expression of $\tilde{g}(x_t)$ in \eqref{eqn:GradientEstimate_Noiseless}, we have that
%\begin{equation}
%\label{eqn:BSM_1}
%\begin{split}
%& \mathbb{E}[\|\tilde{g} (x_t)\|^2] = \mathbb{E}[\frac{1}{\delta^2} \big(f(x_t + \delta u_t) - f(x_{t-1} + \delta u_{t-1})\big)^2 \|u_t\|^2] \\
%& \leq \frac{2}{\delta^2} \mathbb{E}[ \big(f(x_t + \delta u_t) - f(x_{t-1} + \delta u_{t})\big)^2 \|u_t\|^2] + \frac{2}{\delta^2} \mathbb{E}[ \big( f(x_{t-1} + \delta u_{t}) - f(x_{t-1} + \delta u_{t-1})\big)^2 \|u_t\|^2].
%\end{split}
%\end{equation}
\begin{align}
\label{eqn:BSM_1}
\mathbb{E}[\|\tilde{g} (x_t)\|^2] & = \mathbb{E}[\frac{1}{\delta^2} \big(f(x_t + \delta u_t) - f(x_{t-1} + \delta u_{t-1})\big)^2 \|u_t\|^2] & \nonumber \\
& \leq \frac{2}{\delta^2} \mathbb{E}[ \big(f(x_t + \delta u_t) - f(x_{t-1} + \delta u_{t})\big)^2 \|u_t\|^2] & \nonumber  \\
& \quad + \frac{2}{\delta^2} \mathbb{E}[ \big( f(x_{t-1} + \delta u_{t}) - f(x_{t-1} + \delta u_{t-1})\big)^2 \|u_t\|^2]. &
\end{align}
Since function $f \in C^{0,0}$ with Lipschitz constant $L_0$, we obtain that
\begin{equation}
\label{eqn:BSM_2}
\mathbb{E}[\|\tilde{g} (x_t)\|^2] \leq \frac{2 L_0^2}{\delta^2} \mathbb{E}[ \|x_t - x_{t-1}\|^2 \|u_t\|^2 ] + 2L_0^2 \mathbb{E}[\|u_t - u_{t-1}\|^2\|u_t\|^2].
\end{equation}
Since $u_t$ is independently sampled from $x_t - x_{t-1}$, we have that $\mathbb{E}[ \|x_t - x_{t-1}\|^2 \|u_t\|^2 ] = \mathbb{E}[\|x_t - x_{t-1}\|^2] \mathbb{E}[\|u_t\|^2]$. Since $u_t$ is subject to standard multivariate normal distribution, $\mathbb{E}[\|u_t\|^2] = d$. Furthermore, using Lemma 1 in \cite{nesterov2017random}, we get that $\mathbb{E}[\|u_t - u_{t-1}\|^2\|u_t\|^2] \leq 2\mathbb{E}[(\|u_t\|^2 + \|u_{t-1}\|^2)\|u_t\|^2] = 2\mathbb{E}[(\|u_t\|^4] +2\mathbb{E}[ \|u_{t-1}\|^2\|u_t\|^2] \leq 4(d+4)^2$. Plugging these bounds into inequality~\eqref{eqn:BSM_2}, we have that
\begin{equation*}
\label{eqn:BSM_3}
\mathbb{E}[\|\tilde{g} (x_t)\|^2] \leq \frac{2 d L_0^2}{\delta^2} \mathbb{E}[ \|x_t - x_{t-1}\|^2] + 8L_0^2 (d+4)^2.
\end{equation*}
Since $x_t = x_{t-1} - \eta \tilde{g}(x_{t-1})$, we get that
\begin{equation*}
\label{eqn:BSM_4}
\mathbb{E}[\|\tilde{g} (x_t)\|^2] \leq \frac{2 d L_0^2 \eta^2}{\delta^2} \mathbb{E}[ \|\tilde{g}(x_{t-1})\|^2] + 8L_0^2 (d+4)^2.
\end{equation*}

Next, we show the bound when we have the additional smoothness condition $f(x) \in C^{1,1}$ with constant $L_1$. Given the gradient estimate in \eqref{eqn:GradientEstimate_Noiseless}, we have that
\begin{equation}
\label{eqn:BSM_5}
\mathbb{E}[ \| \tilde{g}(x_t) \|^2 ] \leq \mathbb{E}[ \frac{ (f(x_t + \delta u_t) - f(x_{t-1} + \delta u_{t-1}) )^2 }{\delta^2} \|u_t\|^2 ].
\end{equation}
Next, we bound the term $( f(x_t + \delta u_t) - f(x_{t-1} + \delta u_{t-1}) )^2$. Adding and subtracting $f(x_{t-1} + \delta u_{t})$ inside the square, and applying the inequality $(a + b)^2 \leq 2a^2 + 2b^2$, we can obtain
%\begin{equation}
%\label{eqn:BSM_6}
%( f(x_t + \delta u_t) - f(x_{t-1} + \delta u_{t-1}) )^2 \leq 2( f(x_t + \delta u_t) - f(x_{t-1} + \delta u_{t}) )^2 + 2( f(x_{t-1} + \delta u_{t}) - f(x_{t-1} + \delta u_{t-1}) )^2.
%\end{equation} 
\begin{align}
\label{eqn:BSM_6}
( f(x_t + \delta u_t) - f(x_{t-1} + \delta u_{t-1}) )^2 \leq & 2( f(x_t + \delta u_t) - f(x_{t-1} + \delta u_{t}) )^2 &  \nonumber \\
& + 2( f(x_{t-1} + \delta u_{t}) - f(x_{t-1} + \delta u_{t-1}) )^2. &
\end{align} 
Since the function $f(x)$ is also Lipschitz continuous with constant $L_0$, we get that
\begin{equation}
\label{eqn:BSM_7}
( f(x_t + \delta u_{t}) - f(x_{t-1} + \delta u_{t}) )^2 \leq L_0^2 \|x_t - x_{t-1}\|^2 = L_0^2 \eta^2 \|\tilde{g}(x_{t-1})\|^2.
\end{equation}
Next, we bound the term $( f(x_{t-1} + \delta u_t) - f(x_{t-1} + \delta u_{t-1}) )^2$. Adding and subtracting $f(x_{t-1})$, $\langle \nabla f(x_{t-1}), \delta u_t \rangle$ and $\langle \nabla f(x_{t-1}), \delta u_{t-1} \rangle$ inside the square term, we have that
%\begin{equation}
%\label{eqn:BSM_8}
%\begin{split}
%( f(x_{t-1} + \delta u_t) - f(x_{t-1} + \delta u_{t-1}) )^2 \leq & 2\langle \nabla f(x_{t-1}), \delta (u_t - u_{t-1}) \rangle^2 + 4(f(x_{t-1} + \delta u_t) - f(x_{t-1}) - \langle \nabla f(x_{t-1}), \delta u_t \rangle)^2 \\
%& + 4(f(x_{t-1} + \delta u_{t-1}) - f(x_{t-1}) - \langle \nabla f(x_{t-1}), \delta u_{t-1} \rangle)^2.
%\end{split}
%\end{equation}
\begin{align}
\label{eqn:BSM_8}
& ( f(x_{t-1} + \delta u_t) - f(x_{t-1} + \delta u_{t-1}) )^2 & \nonumber \\
\leq & \; 2\langle \nabla f(x_{t-1}), \delta (u_t - u_{t-1}) \rangle^2 + 4(f(x_{t-1} + \delta u_t) - f(x_{t-1}) - \langle \nabla f(x_{t-1}), \delta u_t \rangle)^2 & \nonumber \\
& + 4(f(x_{t-1} + \delta u_{t-1}) - f(x_{t-1}) - \langle \nabla f(x_{t-1}), \delta u_{t-1} \rangle)^2. &
\end{align}
Since $f(x) \in C^{1,1}$ with constant $L_1$, we get that $| f(x_{t-1} + \delta u_t) - f(x_{t-1}) - \langle \nabla f(x_{t-1}), \delta u_t \rangle | \leq \frac{1}{2} L_1 \delta^2 \|u_t\|^2$, according to (6) in \cite{nesterov2017random}. And similarly, we also have $|f(x_{t-1} + \delta u_{t-1}) - f(x_{t-1}) - \langle \nabla f(x_{t-1}), \delta u_{t-1} \rangle| \leq \frac{1}{2} L_1 \delta^2 \|u_{t-1}\|^2$. Substituting these inequalities into \eqref{eqn:BSM_8}, we obtain that
\begin{equation}
\label{eqn:BSM_9}
( f(x_{t-1} + \delta u_t) - f(x_{t-1} + \delta u_{t-1}) )^2 \leq 2\langle \nabla f(x_{t-1}), \delta (u_t - u_{t-1}) \rangle^2  + L_1^2 \delta^4 \|u_t\|^4 + L_1^2 \delta^4 \|u_{t-1}\|^4.
\end{equation}
Moreover, substituting the inequalities~\eqref{eqn:BSM_7} and \eqref{eqn:BSM_9} in the upper bound in \eqref{eqn:BSM_6}, we get that
%\begin{equation}
%\label{eqn:BSM_10}
%( f(x_t + \delta u_t) - f(x_{t-1} + \delta u_{t-1}) )^2  \leq 2 L_0^2 \eta^2 \|\tilde{g}(x_{t-1})\|^2 +  4\langle \nabla f(x_{t-1}), \delta (u_t - u_{t-1}) \rangle^2  + 2L_1^2 \delta^4 \|u_t\|^4 + 2L_1^2 \delta^4 \|u_{t-1}\|^4
%\end{equation}
\begin{align}
\label{eqn:BSM_10}
( f(x_t + \delta u_t) - f(x_{t-1} + \delta u_{t-1}) )^2  \leq & 2 L_0^2 \eta^2 \|\tilde{g}(x_{t-1})\|^2 +  4\langle \nabla f(x_{t-1}), \delta (u_t - u_{t-1}) \rangle^2  & \nonumber \\
& + 2L_1^2 \delta^4 \|u_t\|^4 + 2L_1^2 \delta^4 \|u_{t-1}\|^4 &
\end{align}

Using the bound \eqref{eqn:BSM_10} in inequality~\eqref{eqn:BSM_5}, and applying the bounds $\mathbb{E}[ \|u_t\|^6 ] \leq (d+6)^3$ and $\mathbb{E}[\|u_{t-1}\|^4 \|u_t\|^2] \leq (d+6)^3$, we have that
\begin{equation}
\label{eqn:BSM_11}
\mathbb{E}[ \| \tilde{g}(x_t) \|^2 ] \leq \frac{2d L_0^2 \eta^2}{\delta^2}\mathbb{E}[ \| \tilde{g}(x_{t-1}) \|^2 ] + 4 \mathbb{E}[ \langle \nabla f(x_{t-1}), u_t - u_{t-1} \rangle^2 \|u_t\|^2 ] + 4L_1^2 (d+6)^3 \delta^2 .
\end{equation}
Since $\langle \nabla f(x_{t-1}), u_t - u_{t-1} \rangle^2 \leq 2 \langle \nabla f(x_{t-1}), u_t \rangle^2 + 2\langle \nabla f(x_{t-1}), u_{t-1} \rangle^2$, we get that
\begin{equation}
\label{eqn:BSM_12}
\mathbb{E}[ \langle \nabla f(x_{t-1}), u_t - u_{t-1} \rangle^2 \|u_t\|^2 ] \leq 2 \mathbb{E}[ \langle \nabla f(x_{t-1}), u_t \rangle^2 \|u_t\|^2 ]+ 2 \mathbb{E}[ \langle \nabla f(x_{t-1}), u_{t-1} \rangle^2 \|u_t\|^2 ].
\end{equation}
For the term $\mathbb{E}[ \langle \nabla f(x_{t-1}), u_{t-1} \rangle^2 \|u_t\|^2 ]$, we have that $\mathbb{E}[ \langle \nabla f(x_{t-1}), u_{t-1} \rangle^2 \|u_t\|^2 ] \leq \mathbb{E}[ \|\nabla f(x_{t-1})\|^2 \|u_{t-1}\|^2 \|u_t\|^2 ] \leq d^2 \mathbb{E}[ \|\nabla f(x_{t-1})\|^2 ]$. For the term $\mathbb{E}[ \langle \nabla f(x_{t-1}), u_t \rangle^2 \|u_t\|^2 ]$, according to Theorem 3 in \cite{nesterov2017random}, we have a stronger bound $\mathbb{E}[ \langle \nabla f(x_{t-1}), u_t \rangle^2 \|u_t\|^2 ] \leq (d + 4)  \mathbb{E}[ \|\nabla f(x_{t-1})\|^2 ]$. Substituting these bounds into \eqref{eqn:BSM_12}, and because $d^2 + d + 4 \leq (d + 4)^2$, we have that
\begin{equation}
\label{eqn:BSM_13}
\mathbb{E}[ \langle \nabla f(x_{t-1}), u_t - u_{t-1} \rangle^2 \|u_t\|^2 ] \leq 2(d+4)^2 \mathbb{E}[ \|\nabla f(x_{t-1})\|^2 ].
\end{equation}
Substituting the bound \eqref{eqn:BSM_13} into inequality~\eqref{eqn:BSM_11}, we complete the proof.

\section{Proof of Theorem~\ref{thm:Nonconvex_Noiseless}}
\label{sec:NonsmoothNonconvex_Det}
Since we have that $f(x) \in C^{0,0}$, according to Lemma~\ref{lem:GaussianApprox}, the function $f_\delta(x)$ has $L_1(f_\delta)$-Lipschitz continuous gradient where $L_1(f_\delta) = \frac{\sqrt{d}}{\delta} L_0$. Furthermore, according to Lemma 1.2.3 in \cite{nesterov2013introductory}, we can get the following inequality
\begin{equation}
\label{eqn:Inequality_1}
\begin{split}
f_\delta(x_{t+1}) &\leq f_\delta(x_{t}) +  \langle \nabla f_\delta(x_t), x_{t+1} - x_t \rangle + \frac{L_1(f_\delta)}{2} \|x_{t+1} - x_t\|^2 \\
& = f_\delta(x_{t}) - \eta \langle \nabla f_\delta(x_t), \tilde{g}(x_t) \rangle + \frac{L_1(f_\delta) \eta^2}{2} \|\tilde{g} (x_t)\|^2 \\
& = f_\delta(x_{t}) - \eta \langle \nabla f_\delta(x_t), \Delta_t \rangle - \eta \|\nabla f_\delta(x_t)\|^2 + \frac{L_1(f_\delta) \eta^2}{2} \|\tilde{g}(x_t)\|^2,
\end{split}
\end{equation}
where $\Delta_t = \tilde{g}(x_t) - \nabla f_\delta(x_t)$. According to Lemma~\ref{lem:UnbiasedEstimate_Noiseless}, we can get that $\mathbb{E}_{u_t} [ \tilde{g}(x_t) ] = \nabla f_\delta(x_t)$. Therefore, taking expectation over $u_t$ on both sides of inequality~\eqref{eqn:Inequality_1} and rearranging terms, we have that
\begin{equation}
\label{eqn:Inequality_2}
\eta \mathbb{E}[\|\nabla f_\delta(x_t)\|^2 ] \leq \mathbb{E}[f_\delta(x_t)] - \mathbb{E}[f_\delta(x_{t+1})] + \frac{L_1(f_\delta) \eta^2}{2} \mathbb{E}[ \|\tilde{g}(x_t)\|^2].
\end{equation}

Telescoping above inequalities from $t = 0$ to $T-1$ and dividing both sides by $\eta$, we obtain that
\begin{equation}
\label{eqn:Inequality_3}
\begin{split}
\sum_{t = 0}^{T-1} \mathbb{E}[\|\nabla f_\delta(x_t)\|^2 ] & \leq \frac{\mathbb{E}[f_\delta(x_0)] - \mathbb{E}[f_\delta(x_{T})]}{\eta} + \frac{L_1(f_\delta) \eta}{2} \sum_{t = 0}^{T-1} \mathbb{E}[\|\tilde{g}(x_t)\|^2] \\
& \leq \frac{\mathbb{E}[f_\delta(x_0)] - f_\delta^\ast}{\eta} + \frac{L_1(f_\delta) \eta}{2} \sum_{t = 0}^{T-1} \mathbb{E}[\|\tilde{g}(x_t)\|^2],
\end{split}
\end{equation}
where $f_\delta^\ast$ is the lower bound of the smoothed function $f_\delta(x)$. $f_\delta^\ast$ must exist because we assume the orignal function $f(x)$ is lower bounded and the smoothed function has a bounded distance from $f(x)$ due to Lemma~\ref{lem:GaussianApprox}.

Recall the contraction result of the second moment $\mathbb{E}[ \|\tilde{g}(x_t)\|^2] $ in Lemma~\ref{lem:BoundSecondMoment_Det} when $f(x) \in C^{0,0}$. Denote the contraction rate $\frac{2 d L_0^2 \eta^2}{\delta^2}$ as $\alpha$ and the constant perturbation term $M = 8L_0^2 (d+4)^2$. Then, we get that
\begin{equation}
\mathbb{E}[\|\tilde{g} (x_t)\|^2] \leq \alpha^t \mathbb{E}[\|\tilde{g}(x_0)\|^2] + \frac{1 - \alpha^t}{1 - \alpha} M.
\end{equation}
Summing the above inequality over time, we obtain
\begin{equation}
\label{eqn:Inequality_6}
\begin{split}
\sum_{t = 0}^{T-1} \|\tilde{g}(x_t)\|^2 & \leq \frac{1 - \alpha^{T}}{1 - \alpha} \mathbb{E}[ \|\tilde{g}(x_{0})\|^2] + \sum_{t = 0}^{T-1} \big( \frac{1 - \alpha^t}{1 - \alpha} M \big) \\
& \leq  \frac{1}{1 - \alpha} \mathbb{E}[ \|\tilde{g}(x_{0})\|^2] + \frac{1}{1 - \alpha} M T.
\end{split}
\end{equation}
Plugging the bound in \eqref{eqn:Inequality_6} into inequality~\eqref{eqn:Inequality_3}, and since $L_1(f_\delta) = \frac{\sqrt{d}}{\delta} L_0$, we have that
\begin{equation}
\label{eqn:Inequality_7}
\sum_{t = 0}^{T-1} \mathbb{E}[\|\nabla f_\delta(x_t)\|^2 ] \leq \frac{\mathbb{E}[f_\delta(x_0)] - f_\delta^\ast}{\eta} + \frac{d^\frac{1}{2} L_0 \eta}{\delta}  \big(\frac{1}{1 - \alpha} \mathbb{E}[ \|\tilde{g}(x_{0})\|^2] + \frac{1}{1 - \alpha} 8 L_0^2 (d+4)^2 T\big) .
\end{equation}
To fullfill the requirement that $|f(x) - f_\delta(x)| \leq \epsilon_f$, we set the exporation parameter $\delta = \frac{\epsilon_f}{d^\frac{1}{2} L_0}$. In addition, let the stepsize be $\eta = \frac{\sqrt{\epsilon_f} }{  2d L_0^2 T^{\frac{1}{2}}}$. 
We have that $\alpha = \frac{1}{2T \epsilon_f} \leq \frac{1}{2}$ and $\frac{1}{1 - \alpha} \leq 2$, when $T \geq \frac{1}{\epsilon_f}$. Plugging the choices of $\eta$ and $\delta$ into inequality~\eqref{eqn:Inequality_7}, we obtain that
\begin{equation*}
\sum_{t = 0}^{T-1} \mathbb{E}[\|\nabla f_\delta(x_t)\|^2 ] \leq 2 L_0^2 \big( \mathbb{E}[f_\delta(x_t)] - f_\delta^\ast \big) \frac{d}{\sqrt{\epsilon_f}}\sqrt{T} + \mathbb{E}[ \|\tilde{g}(x_{0})\|^2]  + 8L_0^2 \frac{(d+4)^2}{\sqrt{\epsilon_f}} \sqrt{T}.
\end{equation*}
Dividing both sides of above inequality by $T$, we complete the proof.

\section{Proof of Theorem~\ref{thm:Nonconvex_NoiselessSmooth}}
\label{sec:SmoothNonconvex_Det}
Following the same process in the beginning of the proof of Theorem~\ref{thm:Nonconvex_Noiseless}, we can get
\begin{equation}
\label{eqn:Pf_3.4_1}
\sum_{t = 0}^{T-1} \mathbb{E}[\|\nabla f_\delta(x_t)\|^2 ] \leq \frac{\mathbb{E}[f_\delta(x_0)] - f_\delta^\ast}{\eta} + \frac{L_1\eta}{2} \sum_{t = 0}^{T-1} \mathbb{E}[ \|\tilde{g}(x_t)\|^2 ].
\end{equation}
Since $\frac{1}{2} \mathbb{E}[ \|\nabla f(x_t)\|^2 ] \leq \mathbb{E}[ \|\nabla f_\delta(x_t)\|^2 ] + \mathbb{E}[ \|\nabla f(x_t) - \nabla f_\delta(x_t) \|^2 ]$, and according to the bound~\eqref{eqn:Pf_3.4_1} and Lemma~\ref{lem:GaussianApprox}, we have that
\begin{equation}
\label{eqn:Pf_3.4_2}
	\frac{1}{2} \sum_{t=0}^{T-1} \|\mathbb{E}[ \|\nabla f(x_t)\|^2 \|] \leq \frac{\mathbb{E}[f_\delta(x_0)] - f_\delta^\ast}{\eta} + \frac{L_1\eta}{2} \sum_{t = 0}^{T-1} \mathbb{E}[\|\tilde{g}(x_t)\|^2] + L_1^2 (d+3)^3 \delta^2 T.
\end{equation}
In addition, similar to the process to derive the bound in \eqref{eqn:Inequality_6}, according to Lemma~\ref{lem:BoundSecondMoment_Det}, when $f(x) \in C^{1,1}$, we can get that
\begin{equation}
\label{eqn:Pf_3.4_3}
	\sum_{t = 0}^{T-1} \|\tilde{g}(x_t)\|^2  \leq \frac{1}{1 - \alpha}  \mathbb{E}[ \|\tilde{g}(x_0)\|^2 ] + \frac{8}{1 - \alpha} (d+4)^2 \sum_{t = 0}^{T-1} \|\nabla f(x_t)\|^2 + \frac{4}{1 - \alpha} L_1^2 (d+6)^3 \delta^2 T.
\end{equation}
Plugging the bound~\eqref{eqn:Pf_3.4_3} into \eqref{eqn:Pf_3.4_2}, we have that 
\begin{equation}
\label{eqn:Pf_3.5_4}
\begin{split}
\frac{1}{2} \sum_{t=0}^{T-1} \|\mathbb{E}[ \|\nabla f(x_t)\|^2 \|] \leq & \frac{\mathbb{E}[f_\delta(x_0)] - f_\delta^\ast}{\eta} + \frac{L_1\eta}{2} \big( \frac{1}{1 - \alpha}  \mathbb{E}[ \|\tilde{g}(x_0)\|^2 ] + \frac{4}{1 - \alpha} L_1^2 (d+6)^3 \delta^2 T \\ 
& + \frac{8}{1 - \alpha} (d+4)^2 \sum_{t = 0}^{T-1} \mathbb{E}[\|\nabla f(x_t)\|^2] \big) + L_1^2 (d+3)^3 \delta^2 T.
\end{split}
\end{equation}
Recalling that $\tilde{L} = \max\{32 L_1, 2L_0\}$, let $\eta = \frac{1}{\tilde{L} (d+4)^2 T^\frac{1}{3}}$ and $\delta = \frac{1}{\sqrt{d} T^\frac{1}{3}}$, and we have that $\alpha = 2d L_0^2 \frac{\eta^2}{\delta^2} \leq \frac{1}{2}$. In addition, the coefficient before the term $ \|\nabla f(x_t)\|^2$ in the upper bound above $\frac{L_1 \eta}{2} \frac{8}{1 - \alpha} (d+4)^2 \leq \frac{1}{4}$. Therefore, we obtain that
\begin{equation}
\label{eqn:Pf_3.5_6}
\begin{split}
\frac{1}{4} \sum_{t=0}^{T-1} \|\mathbb{E}[ \|\nabla f(x_t)\|^2 \|] \leq & \tilde{L} (\mathbb{E}[f_\delta(x_0)] - f_\delta^\ast)(d+4)^2 T^\frac{1}{3} + \frac{1}{32 (d+4)^2 T^\frac{1}{3}} \mathbb{E}[ \|\tilde{g}(x_0)\|^2 ] \\
& + \frac{L_1^2}{8} \frac{(d+6)^3 }{(d+4)^2 d} + L_1^2 \frac{(d+3)^3}{d} T^\frac{1}{3}.
\end{split}
\end{equation}
Dividing both sides of above inequality by $T$, we complete the proof.

\section{Proof of Theorem~\ref{thm:Convex_Noiseless}}
\label{sec:Convex_Det}

First, according to iteration~\eqref{eqn:SGD}, we have that
\begin{equation}
	\|x_{t+1} - x^*\|^2 \leq \|x_t - \eta \widetilde{g}(x_t) -x^*\|^2 = \|x_{t} - x^*\|^2 -2\eta \inner{\widetilde{g}(x_t)}{x_t - x^*} + \eta^2 \|\widetilde{g}(x_t)\|^2.
\end{equation}
Taking expectation on both sides, and since $\mathbb{E} [\tilde{g}(x_t)] = \nabla f_\delta (x_t)$, we obtain that
\begin{equation}
\label{eqn:Pf_3.5_1}
\mathbb{E}[ \|x_{t+1} - x^*\|^2 ] \leq \mathbb{E}[ \|x_{t} - x^\ast\|^2 ] -2\eta \langle \nabla f_\delta(x_t) , x_t - x^\ast \rangle + \eta^2 \mathbb{E}[\|\tilde{g}(x_t)\|^2].
\end{equation}
Due to the convexity, we have that $\langle \nabla f_\delta(x_t) , x_t - x^\ast \rangle \geq f_\delta(x_t) - f_\delta(x^\ast)$. Plugging this inequality into \eqref{eqn:Pf_3.5_1}, we have that
\begin{equation}
\label{eqn:Pf_3.5_2}
\mathbb{E}[\|x_{t+1} - x^*\|^2] \leq \mathbb{E}[\|x_{t} - x^\ast\|^2] -2\eta (f_\delta(x_t) - f_\delta(x^\ast))+ \eta^2 \mathbb{E}[ \|\tilde{g}(x_t)\|^2 ].
\end{equation}
When $f(x) \in C^{0,0}$, using Lemma~\eqref{lem:GaussianApprox}, we can replace $f_\delta(x)$ with $f(x)$ in above inequality and get
\begin{equation}
\label{eqn:Pf_3.5_3}
\mathbb{E}[ \|x_{t+1} - x^*\|^2 ] \leq \mathbb{E}[ \|x_{t} - x^\ast\|^2 ] -2\eta (f(x_t) - f(x^\ast))+ \eta^2 \mathbb{E}[ \|\tilde{g}(x_t)\|^2 ] + 4  L_0 \sqrt{d} \delta \eta.
\end{equation}
Rearranging the terms and telescoping from $t = 0$ to $T-1$, we obtain that
\begin{align}
	\sum_{t = 0}^{T-1} \mathbb{E}[f(x_t)] - T f(x^\ast) & \leq \frac{1}{2\eta} (\|x_{0} - x^\ast\|^2 - \mathbb{E}[ \|x_{T} - x^\ast\|^2 ]) + \frac{\eta}{2} \sum_{t = 0}^{T-1} \mathbb{E}[ \|\tilde{g}(x_t)\|^2 ] + 2 L_0 \sqrt{d} \delta T & \nonumber \\
	& \leq \frac{1}{2\eta}  \|x_{0} - x^\ast\|^2  + \frac{\eta}{2} \sum_{t = 0}^{T-1} \mathbb{E}[ \|\tilde{g}(x_t)\|^2 ] + 2 L_0 \sqrt{d} \delta T &
\end{align}
Since function $f(x) \in C^{0,0}$, we can plug the bound~\eqref{eqn:Inequality_6} into the above inequality and get that
\begin{equation}
	\sum_{t = 0}^{T-1} \mathbb{E}[ f(x_t)] - T f(x^\ast) \leq \frac{1}{2\eta}  \|x_{0} - x^\ast\|^2  + \frac{\eta}{2 (1-\alpha)} \mathbb{E}[\|\tilde{g}(x_0)\|^2] + \frac{4 \eta}{1-\alpha} L_0^2 (d+4)^2 T + 2 L_0 \sqrt{d} \delta T. 
\end{equation}
Let $\eta = \frac{1}{2 d L_0 \sqrt{T}}$ and $\delta = \frac{1}{\sqrt{T}}$. We have that $\alpha = 2dL_0^2 \frac{\eta^2}{\delta^2} = \frac{1}{2d} \leq \frac{1}{2}$. Therefore, $\frac{1}{1 - \alpha} \leq 2$. Applying this bound and the choice of $\eta$ and $\delta$ into above inequality, we have that
\begin{align}
	\sum_{t = 0}^{T-1} \mathbb{E}[f(x_t)] - T f(x^\ast) \leq & L_0 \|x_{0} - x^\ast\|^2 d\sqrt{T} + \frac{1}{2 d L_0 \sqrt{T}} \mathbb{E}[\|\tilde{g}(x_0)\|^2] & \nonumber \\
	& + 4 L_0 \frac{(d + 4)^2}{d} \sqrt{T} + 2L_0 \sqrt{d} \sqrt{T}. &
\end{align}
Recalling that $f(\bar{x}) \leq \frac{1}{T}\sum_{t = 0}^{T-1} f(x_t)$ due to  convexity and dividing both sides of above inequality by $T$, the proof of the nonsmooth case is complete.

When function $f(x) \in C^{1,1}$, it is straightforward to see that we also have the inequality~\eqref{eqn:Pf_3.5_2}. In addition, according to Lemma~\ref{lem:GaussianApprox}, we can replace $f_\delta(x)$ with $f(x)$ in above inequality and get
\begin{equation}
\label{eqn:Pf_3.5_5}
\mathbb{E}[ \|x_{t+1} - x^*\|^2 ] \leq \mathbb{E}[\|x_{t} - x^\ast\|^2] -2\eta (f(x_t) - f(x^\ast))+ \eta^2 \mathbb{E}[\|\tilde{g}(x_t)\|^2] + 4  L_1 d \delta^2 \eta.
\end{equation}
Similarly to the above analysis, we telescope the above inequality from $t = 0$ to $T-1$, apply the bound on $\sum_{t = 0}^{T-1} \mathbb{E}[\|\tilde{g}(x_t)\|^2]$ in \eqref{eqn:Pf_3.4_3} and obtain that
\begin{align}
	\sum_{t = 0}^{T-1} \mathbb{E}[f(x_t)] - T f(x^\ast) \leq & \; \frac{1}{2\eta}  \|x_{0} - x^\ast\|^2  + \frac{\eta}{2 (1-\alpha)} \mathbb{E}[\|\tilde{g}(x_0)\|^2]  + \frac{2 \eta}{1-\alpha} L_1^2 (d+6)^3 \delta^2 T & \nonumber \\
	&  + \frac{4 \eta}{1-\alpha} (d+4)^2 \sum_{t = 0}^{T-1} \mathbb{E}[\| \nabla f(x_t)\|^2] + 2 L_1 d \delta^2 T. &
\end{align}
Since $f(x) \in C^{1,1}$ is convex, we have that $\| \nabla f(x_t)\|^2 \leq 2L_1 (f(x_t) - f(x^\ast))$ according to (2.1.7) in \cite{nesterov2013introductory}. Applying this bound into the above inequality, we get that
\begin{align}
\sum_{t = 0}^{T-1} \mathbb{E}[f(x_t)] - T f(x^\ast) \leq & \; \frac{1}{2\eta}  \|x_{0} - x^\ast\|^2  + \frac{\eta}{2 (1-\alpha)} \mathbb{E}[\|\tilde{g}(x_0)\|^2]  + \frac{2 \eta}{1-\alpha} L_1^2 (d+6)^3 \delta^2 T  & \nonumber \\
& + \frac{8\eta}{1-\alpha} L_1 (d+4)^2 \big( \sum_{t = 0}^{T-1} \mathbb{E}[f(x_t)] - T f(x^\ast) \big) + 2 L_1 d \delta^2 T. &
\end{align}
Let $\eta = \frac{1}{2 \tilde{L} (d+4)^2 T^{\frac{1}{3}}}$ and $\delta = \frac{\sqrt{d}}{T^{\frac{1}{3}}}$ where $\tilde{L} = \max\{L_0, 16L_1\}$. Then, we have that $\alpha = 2dL_0^2 \frac{\eta^2}{\delta^2} \leq \frac{1}{2(d+4)^4} \leq \frac{1}{2}$. In addition, we have that $\frac{8\eta}{1-\alpha} L_1 (d+4)^2 \leq \frac{1}{2 T^\frac{1}{3}} \leq \frac{1}{2}$. Applying these two bounds into above inequality and rearranging terms, we have that
%\begin{equation}
%\frac{1}{2} \sum_{t = 0}^{T-1} \mathbb{E}[f(x_t)] - T f(x^\ast) \leq \tilde{L} \|x_{0} - x^\ast\|^2 (d+4)^2 T^\frac{1}{3} +  \frac{1}{2 \tilde{L} (d+4)^2 T^{\frac{1}{3}}} \mathbb{E}[\|\tilde{g}(x_0)\|^2] + \frac{L_1}{8} \frac{(d+6)^3d}{(d+4)^2} + 2L_1 d^2 T^\frac{1}{3}.
%\end{equation}
\begin{align}
\frac{1}{2} \sum_{t = 0}^{T-1} \mathbb{E}[f(x_t)] - T f(x^\ast) \leq & \; \tilde{L} \|x_{0} - x^\ast\|^2 (d+4)^2 T^\frac{1}{3} +  \frac{1}{2 \tilde{L} (d+4)^2 T^{\frac{1}{3}}} \mathbb{E}[\|\tilde{g}(x_0)\|^2] & \nonumber \\
& + \frac{L_1}{8} \frac{(d+6)^3d}{(d+4)^2} + 2L_1 d^2 T^\frac{1}{3}. &
\end{align}
Recalling that $f(\bar{x}) \leq \frac{1}{T}\sum_{t = 0}^{T-1} f(x_t)$ due to  convexity and dividing both sides of above inequality by $T$, the proof of the smooth case is complete.

\section{Proof of Lemma~\ref{lem:BoundSecondMoment_Stoch}}
The analysis is similar to the proof in~\Cref{sec:BoundSecondMoment_Det}. First, consider the case when $F(x, \xi) \in C^{0,0}$ with $L_0(\xi)$. According to \eqref{eqn:GradientEstimate_Noise}, we have that
\begin{equation}
\label{eqn:BSM_stoch_1}
\begin{split}
\mathbb{E}[\|\tilde{g} (x_t)\|^2] & = \mathbb{E}[\frac{1}{\delta^2} \big(F(x_t + \delta u_t, \xi_t) - F(x_{t-1} + \delta u_{t-1}, \xi_{t-1})\big)^2 \|u_t\|^2]  \\
& \leq \frac{2}{\delta^2} \mathbb{E}[ \big(F(x_t + \delta u_t, \xi_t) - F(x_{t-1} + \delta u_{t-1}, \xi_t)\big)^2 \|u_t\|^2] \\
& \quad \quad \quad \quad \quad + \frac{2}{\delta^2} \mathbb{E}[ \big( F(x_{t-1} + \delta u_{t-1}, \xi_t) - F(x_{t-1} + \delta u_{t-1}, \xi_{t-1})\big)^2 \|u_t\|^2].
\end{split}
\end{equation}
Using the bound in Assumption~\ref{asmp:BoundedVariance}, we get that $\frac{2}{\delta^2} \mathbb{E}[ \big( F(x_{t-1} + \delta u_{t-1}, \xi_t) - F(x_{t-1} + \delta u_{t-1}, \xi_{t-1})\big)^2 \|u_t\|^2] \leq \frac{8 d \sigma^2}{\delta^2}$. In addition, adding and subtracting $F(x_{t-1} + \delta u_{t}, \xi_{t})$ in $\big(F(x_t + \delta u_t, \xi_t) - F(x_{t-1} + \delta u_{t-1}, \xi_t)\big)^2$ in above inequality, we obtain that
\begin{equation}
\begin{split}
\mathbb{E}[\|\tilde{g} (x_t)\|^2] \leq & \frac{4}{\delta^2} \mathbb{E}[ \big(F(x_t + \delta u_t, \xi_t) - F(x_{t-1} + \delta u_{t}, \xi_t)\big)^2 \|u_t\|^2] \\
& + \frac{4}{\delta^2} \mathbb{E}[ \big( F(x_{t-1} + \delta u_{t}, \xi_t) - F(x_{t-1} + \delta u_{t-1}, \xi_{t})\big)^2 \|u_t\|^2] + \frac{8 d \sigma^2}{\delta^2}.
\end{split}
\end{equation}
Using Assumption~\ref{asmp:BoundedLipschitz}, we can bound the first two items on the right hand side of above inequality following the same procedure after inequality~\eqref{eqn:BSM_2} and get that 
\begin{equation}
	\mathbb{E}[\|\tilde{g} (x_t)\|^2] \leq  \frac{4 d L_0^2 \eta^2}{\delta^2} \mathbb{E}[ \|\tilde{g}(x_{t-1})\|^2] + 16L_0^2 (d+4)^2 + \frac{8 d \sigma^2}{\delta^2}.
\end{equation}
The proof is complete.

\section{Proof of Theorem~\ref{thm:NoisyOnline_Nonconvex}}
When function $F(x) \in C^{0,0}$ with $L_0(\xi)$, using Assumption~\ref{asmp:BoundedLipschitz} and following the same procedure in \Cref{sec:NonsmoothNonconvex_Det}, we have that
\begin{equation}
\label{eqn:Pf_4.4_1}
\sum_{t = 0}^{T-1} \mathbb{E}[\|\nabla f_\delta(x_t)\|^2 ]  \leq \frac{\mathbb{E}[f_\delta(x_0)] - f_\delta^\ast}{\eta} + \frac{L_1(f_\delta) \eta}{2} \sum_{t = 0}^{T-1} \mathbb{E}[\|\tilde{g}(x_t)\|^2],
\end{equation}
where $L_1(f_\delta) = \frac{\sqrt{d}}{\delta} L_0$. 
In addition, according to Lemma~\ref{lem:BoundSecondMoment_Stoch}, we get that
\begin{equation}
	\label{eqn:Pf_4.4_2}
	\sum_{t = 0}^{T-1} \mathbb{E}[  \|\tilde{g}(x_t)\|^2 ] \leq \frac{1}{1 - \alpha} \mathbb{E}[ \|\tilde{g}(x_{0})\|^2] + \frac{16 L_0^2}{1 - \alpha} (d+4)^2 T + \frac{8 \sigma^2}{1 - \alpha}\frac{d}{\delta^2} T,
\end{equation}
where $\alpha =  \frac{4 d L_0^2 \eta^2}{\delta^2}$.
Plugging \eqref{eqn:Pf_4.4_2} into the bound in \eqref{eqn:Pf_4.4_1}, we obtain that
%\begin{equation}
%	\label{eqn:Pf_4.4_3}
%	\sum_{t = 0}^{T-1} \mathbb{E}[\|\nabla f_\delta(x_t)\|^2 ]  \leq \frac{\mathbb{E}[f_\delta(x_0)] - f_\delta^\ast}{\eta} + \frac{\sqrt{d} L_0}{2(1 - \alpha)} \mathbb{E}[ \|\tilde{g}(x_{0})\|^2] \frac{\eta}{\delta} + \frac{8 L_0^3 \sqrt{d}}{1 - \alpha} (d+4)^2 \frac{\eta}{\delta} T + \frac{4 \sigma^2 L_0}{1 - \alpha} d^{1.5} \frac{\eta}{\delta^3} T.
%\end{equation}
\begin{align}
\label{eqn:Pf_4.4_3}
\sum_{t = 0}^{T-1} \mathbb{E}[\|\nabla f_\delta(x_t)\|^2 ]  \leq & \; \frac{\mathbb{E}[f_\delta(x_0)] - f_\delta^\ast}{\eta} + \frac{\sqrt{d} L_0}{2(1 - \alpha)} \mathbb{E}[ \|\tilde{g}(x_{0})\|^2] \frac{\eta}{\delta} & \nonumber \\
& + \frac{8 L_0^3 \sqrt{d}}{1 - \alpha} (d+4)^2 \frac{\eta}{\delta} T + \frac{4 \sigma^2 L_0}{1 - \alpha} d^{1.5} \frac{\eta}{\delta^3} T. &
\end{align}
Similar to \Cref{sec:NonsmoothNonconvex_Det}, to fullfill the requirement that $|f(x) - f_\delta(x)| \leq \epsilon_f$, we set the exporation parameter $\delta = \frac{\epsilon_f}{d^\frac{1}{2} L_0}$. In addition, let the stepsize be $\eta = \frac{\epsilon_f^{1.5} }{  2\sqrt{2} L_0^2 d^{1.5} T^{\frac{1}{2}}}$. 
Then, we have that $\alpha =  \frac{4 d L_0^2 \eta^2}{\delta^2} = \frac{\epsilon_f}{2 d T}\leq \frac{1}{2}$ when $T \geq \frac{1}{d \epsilon_f}$. Therefore, we have that $\frac{1}{1 - \alpha} \leq 2$. Applying this bound and the choices of $\eta$ and $\delta$ into the bound~\eqref{eqn:Pf_4.4_3}, we obtain that 
\begin{equation}
\label{eqn:Pf_4.4_4}
\begin{split}
\sum_{t = 0}^{T-1} \mathbb{E}[\|\nabla f_\delta(x_t)\|^2 ]  \leq & 2\sqrt{2} L_0^2 (\mathbb{E} [ f_\delta(x_0) ] - f_\delta^\ast ) \frac{d^{1.5} \sqrt{T}}{\epsilon_f^{1.5}} + \frac{L_0 \epsilon_f^{0.5} }{2 \sqrt{2dT}} \mathbb{E}[ \|\tilde{g}(x_{0})\|^2] \\
& \quad \quad \quad  + 4 \sqrt{2} L_0^2 \frac{(d+4)^2}{\sqrt{d}} \sqrt{\epsilon_f T} +  2\sqrt{2} \sigma^2 L_0^2 \frac{d^{1.5} \sqrt{T}}{\epsilon_f^{1.5}} .
\end{split}
\end{equation}
Dividing both sides by $T$, the proof for the nonsmooth case is complete.

When function $F(x, \xi) \in C^{1,1}$ with $L_1(\xi)$, according to Assumption~\ref{asmp:BoundedLipschitz}, we also have that $f_\delta(x), f(x) \in C^{1,1}$ with constant $L_1$.  Similarly to the proof in \Cref{sec:SmoothNonconvex_Det},  we get that 
\begin{equation}
\label{eqn:Pf_4.4_5}
\frac{1}{2} \sum_{t=0}^{T-1} \|\mathbb{E}[ \|\nabla f(x)\|^2 \|] \leq \frac{\mathbb{E}[f_\delta(x_0)] - f_\delta^\ast}{\eta} + \frac{L_1\eta}{2} \sum_{t = 0}^{T-1} \mathbb{E}[\|\tilde{g}(x_t)\|^2] + L_1^2 (d+3)^3 \delta^2 T.
\end{equation}
Plugging inequality~\eqref{eqn:Pf_4.4_2} into the above upper bound, we obtain that
\begin{equation}
	\begin{split}
	\frac{1}{2} \sum_{t=0}^{T-1} \|\mathbb{E}[ \|\nabla f(x)\|^2 \|] \leq & \frac{\mathbb{E}[f_\delta(x_0)] - f_\delta^\ast}{\eta} + \frac{L_1\eta}{2(1 - \alpha)} \mathbb{E}[ \|\tilde{g}(x_{0})\|^2] + \frac{8 L_0^2 L_1 }{1 - \alpha} (d+4)^2 \eta T \\ 
	& + \frac{4 L_1 \sigma^2}{1 - \alpha}\frac{d\eta}{\delta^2} T + L_1^2 (d+3)^3 \delta^2 T.
	\end{split}
\end{equation}
Let $\eta = \frac{1}{2 \sqrt{2} L_{0} d^{\frac{4}{3}} T^{\frac{2}{3}}}$ and $\delta = \frac{1}{ d^{\frac{5}{6}} T^\frac{1}{6}}$. Then, $\alpha = \frac{4 d L_0^2 \eta^2}{\delta^2} = \frac{1}{2 T} \leq \frac{1}{2}$ and $\frac{1}{1 - \alpha} \leq 2$. Plugging these results into the above inequality, we get that
\begin{equation}
\begin{split}
\frac{1}{2} \sum_{t=0}^{T-1} \|\mathbb{E}[ \|\nabla f(x)\|^2 \|] \leq & 2\sqrt{2} L_0 (\mathbb{E}[f_\delta(x_0)] - f_\delta^\ast) d^{\frac{4}{3}} T^\frac{2}{3} + \frac{L_1}{2 \sqrt{2} L_{0} d^{\frac{4}{3}} T^{\frac{2}{3}}} \mathbb{E}[ \|\tilde{g}(x_{0})\|^2] \\ 
& + 4\sqrt{2} L_0 L_1 \frac{(d+4)^2}{d^\frac{4}{3}} T^\frac{1}{3} + \frac{2\sqrt{2} L_1 \sigma^2}{L_0 d^\frac{1}{3}} T^\frac{1}{3} + L_1^2 \frac{(d+3)^3}{d^\frac{5}{3}}  T^\frac{2}{3}.
\end{split}
\end{equation}
Dividing both sides by $T$, the proof for the smooth case is complete.

\section{Proof of Theorem~\ref{thm:NoisyOnline_Convex}}

When the function $f(x) \in C^{0,0}$ with constant $L_0(\xi)$ is convex, we can follow the same procedure as in \Cref{sec:Convex_Det} and get that
\begin{equation}
	\sum_{t = 0}^{T-1} \mathbb{E}[f(x_t)] - T f(x^\ast) \leq \frac{1}{2\eta}  \|x_{0} - x^\ast\|^2  + \frac{\eta}{2} \sum_{t = 0}^{T-1} \mathbb{E}[\|\tilde{g}(x_t)\|^2] + 2 L_0 \sqrt{d} \delta T.
\end{equation}
Plugging the bound \eqref{eqn:Pf_4.4_2} into above inequality, we have that
%\begin{equation}
%	\sum_{t = 0}^{T-1} \mathbb{E}[f(x_t)] - T f(x^\ast) \leq \frac{1}{2\eta}  \|x_{0} - x^\ast\|^2  + \frac{\eta}{2(1 - \alpha)} \mathbb{E}[ \|\tilde{g}(x_{0})\|^2] + \frac{8 L_0^2}{1 - \alpha} (d+4)^2 \eta T + \frac{4 \sigma^2}{1 - \alpha}\frac{d\eta}{\delta^2} T + 2 L_0 \sqrt{d} \delta T.
%\end{equation}
\begin{align}
\sum_{t = 0}^{T-1} \mathbb{E}[f(x_t)] - T f(x^\ast) \leq & \; \frac{1}{2\eta}  \|x_{0} - x^\ast\|^2  + \frac{\eta}{2(1 - \alpha)} \mathbb{E}[ \|\tilde{g}(x_{0})\|^2] + \frac{8 L_0^2}{1 - \alpha} (d+4)^2 \eta T & \nonumber \\
& + \frac{4 \sigma^2}{1 - \alpha}\frac{d\eta}{\delta^2} T + 2 L_0 \sqrt{d} \delta T. &
\end{align}
Let $\eta = \frac{1}{2\sqrt{2} L_0 \sqrt{d} T^{\frac{3}{4}}}$ and $\delta = \frac{1}{T^{\frac{1}{4}}}$. Then, we have that $\alpha = \frac{4 d L_0^2 \eta^2}{\delta^2} = \frac{1}{2T} \leq \frac{1}{2}$. Plugging these results into the above inequality, we get that
\begin{equation}
\begin{split}
\sum_{t = 0}^{T-1} \mathbb{E}[f(x_t)] - T f(x^\ast) \leq & \sqrt{2} L_0 \|x_{0} - x^\ast\|^2 \sqrt{d} T^\frac{3}{4} + \frac{1}{2\sqrt{2} L_0 \sqrt{d} T^{\frac{3}{4}}} \mathbb{E}[ \|\tilde{g}(x_{0})\|^2] \\ 
& + 4\sqrt{2} L_0 \frac{(d+4)^2}{\sqrt{d}} T^\frac{1}{4} + \frac{2\sqrt{2} \sigma^2}{L_0} \sqrt{d} T^\frac{3}{4} + 2 L_0 \sqrt{d} T^\frac{3}{4}.
\end{split}
\end{equation}
Dividing both sides by $T$, the proof for the nonsmooth case is complete.

When the function $f(x) \in C^{1,1}$ with constant $L_1(\xi)$, we can also get the inequality~\eqref{eqn:Pf_3.5_5} in \Cref{sec:Convex_Det}. Telescoping this inequality from $t = 0$ to $T-1$ and rearranging terms, we obtain
\begin{equation}
\begin{split}
\sum_{t = 0}^{T-1} \mathbb{E}[f(x_t)] - T f(x^\ast) \leq \frac{1}{2\eta}  \|x_{0} - x^\ast\|^2  + \frac{\eta}{2} \sum_{t = 0}^{T-1} \mathbb{E}[\|\tilde{g}(x_t)\|^2] + 2 L_1 d \delta^2 T.
\end{split}
\end{equation}
Plugging the bound \eqref{eqn:Pf_4.4_2} into above inequality, we have that
%\begin{equation}
%\sum_{t = 0}^{T-1} \mathbb{E}[f(x_t)] - T f(x^\ast) \leq \frac{1}{2\eta}  \|x_{0} - x^\ast\|^2  + \frac{\eta}{2(1 - \alpha)} \mathbb{E}[ \|\tilde{g}(x_{0})\|^2] + \frac{8 L_0^2}{1 - \alpha} (d+4)^2 \eta T + \frac{4 \sigma^2}{1 - \alpha}\frac{d\eta}{\delta^2} T + 2 L_1 d \delta^2 T.
%\end{equation}
\begin{align}
\sum_{t = 0}^{T-1} \mathbb{E}[f(x_t)] - T f(x^\ast) \leq &\; \frac{1}{2\eta}  \|x_{0} - x^\ast\|^2  + \frac{\eta}{2(1 - \alpha)} \mathbb{E}[ \|\tilde{g}(x_{0})\|^2] + \frac{8 L_0^2}{1 - \alpha} (d+4)^2 \eta T & \nonumber \\
& + \frac{4 \sigma^2}{1 - \alpha}\frac{d\eta}{\delta^2} T + 2 L_1 d \delta^2 T. &
\end{align}
Let $\eta = \frac{1}{2\sqrt{2} L_0 d^\frac{2}{3} T^{\frac{2}{3}}}$ and $\delta = \frac{1}{  d^\frac{1}{6} T^{\frac{1}{6}}}$. Then, we have that $\alpha = \frac{4 d L_0^2 \eta^2}{\delta^2} = \frac{1}{2T} \leq \frac{1}{2}$. Plugging these parameters into above inequality, we get that
\begin{equation}
\begin{split}
\sum_{t = 0}^{T-1} \mathbb{E}[f(x_t)] - T f(x^\ast) \leq &\; \sqrt{2} L_0 \|x_{0} - x^\ast\|^2 d^\frac{2}{3} T^\frac{2}{3}+ \frac{1}{2\sqrt{2} L_0 d^\frac{2}{3} T^{\frac{2}{3}}} \mathbb{E}[ \|\tilde{g}(x_{0})\|^2] \\
& + 4\sqrt{2} L_0 \frac{(d+4)^2}{d^\frac{2}{3}}T^\frac{1}{3} + \frac{2\sqrt{2} \sigma^2}{L_0} d^\frac{2}{3} T^\frac{2}{3} + 2 L_1  d^\frac{2}{3} T^\frac{2}{3} .
\end{split}
\end{equation}
Dividing both sides by $T$, the proof for the smooth case is complete.

\section{Analysis of SGD with Mini-batch Residual Feedback}

In this section, we analyze the query complexity of SGD with the mini-batch residual feedback. First, we make some additional assumptions.
 
\begin{asmp}
	\label{asmp:BoundedVariance_Gradient}
	When function $F(x, \xi) \in C^{1,1}$, we assume that
	\begin{equation*}
		\label{eqn:BoundedVariance}
		\mathbb{E}_\xi [ \| \nabla F(x, \xi) - \mathbb{E}[ \nabla F(x, \xi)] \|^2 ] \leq \sigma_g^2.
	\end{equation*}
\end{asmp}
Before presenting the main results, we first establish some important lemmas. 
The following lemma provides a characterization for the estimation variance of the estimator $\widetilde{g}_b(x_t)$.

\begin{lem}\label{le:variance11}
	When function $F(x, \xi) \in C^{0,0}$ with constant $L_0(\xi)$, given Assumptions~\ref{asmp:BoundedVariance} and \ref{asmp:BoundedLipschitz}, we have that
	\begin{align}
	\mathbb{E} \|\widetilde g_b(x_t)\|^2  \leq  \frac{4(d+2)L_0^2}{\delta^2}\mathbb{E}\|x_t-x_{t-1}\|^2 + 16L_0^2(d+4)^2  + \frac{8(d+2)\sigma^2}{\delta^2 b}.
	\end{align}
	
	Furthermore, when function $F(x, \xi) \in C^{1,1}$ with constant $L_1(\xi)$, given Assumptions~\ref{asmp:BoundedVariance}, \ref{asmp:BoundedLipschitz} and \ref{asmp:BoundedVariance_Gradient}, we have that 
	\begin{align*}
	\mathbb{E} \|\widetilde g_b(x_t)\|^2 \leq &12L^2_1\delta^2(d+6)^3  + \frac{6 (d+2) L_0^2\eta^2}{\delta^2}\mathbb{E} \|\widetilde g_b(x_{t-1})\|^2 \nonumber
	\\ &  +24(d+4)\mathbb{E}(\|\nabla f(x_t) \|^2+ \|\nabla f(x_{t-1})\|^2) + \frac{48(d+4)\sigma_g^2}{b}+ \frac{8(d+2)\sigma^2}{\delta^2 b}.
	\end{align*}	
\end{lem}

\begin{proof}
	When function $F(x, \xi) \in C^{0,0}$, based on the definition of $\widetilde g(x_t)$, we have
	\begin{align*}
 \|\widetilde g_b(x_t) \|^2 = & \frac{1}{\delta^2 b^2}|F(x_t+\delta u_t, \xi_{1:b}) -F(x_{t-1}+\delta u_{t-1},\xi_{1:b}) & \nonumber \\
 & \quad \quad \quad + F(x_{t-1}+\delta u_{t-1};\xi_{1:b}) - F(x_{t-1}+\delta u_{t-1},\xi_{1:b}')  |^2 \|u_t\|^2\nonumber \\
  \leq& \frac{2}{\delta^2 b^2}\big(|F(x_t+\delta u_t,\xi_{1:b}) - F(x_{t-1}+\delta u_{t-1},\xi_{1:b})|^2 + & \nonumber \\
  & \quad \quad \quad  |F(x_{t-1}+\delta u_{t-1},\xi_{1:b})-F(x_{t-1}+\delta u_{t-1},\xi_{1:b}')  |^2 \big)\|u_t\|^2 \nonumber
	\\ \leq &\frac{4L_0^2}{\delta^2}\|x_t-x_{t-1}\|^2\|u_t\|^2+4L_0^2\|u_{t}- u_{t-1}\|^2\|u_t\|^2  & \nonumber \\ 
	& +\frac{2}{\delta^2 b^2} |F(x_{t-1} +\delta u_{t-1},\xi_{1:b})-F(x_{t-1}+\delta u_{t-1},\xi_{1:b}')  |^2\|u_t\|^2. & \nonumber
	\end{align*}
	Taking expectation over the above inequality yields
	\begin{align}\label{pqo}
	& \mathbb{E} \|\widetilde g_b(x_t)\|^2 \leq \frac{4L_0^2}{\delta^2}\mathbb{E}\big(\|x_t-x_{t-1}\|^2\|u_t\|^2\big)+4L_0^2\mathbb{E}\big(\|u_{t}- u_{t-1}\|^2\|u_t\|^2 \big) \nonumber
	\\&\quad \quad \quad \quad \quad \quad +\frac{2}{\delta^2 b^2} \mathbb{E}\big(|F(x_{t-1}+\delta u_{t-1},\xi_{1:b})-F(x_{t-1}+\delta u_{t-1},\xi_{1:b}')  |^2\|u_t\|^2 \big)\nonumber
	\\ \leq & \frac{4L_0^2}{\delta^2}\mathbb{E}\big(\|x_t-x_{t-1}\|^2\mathbb{E}_{u_t}\|u_t\|^2 \big) + 8L_0^2\mathbb{E}\big(\|u_{t}\|^4+\|u_{t-1}\|^2\|u_t\|^2 \big) \nonumber
		\\&\quad \quad  \quad+\frac{2}{\delta^2} \mathbb{E}\big(|F(x_{t-1}+\delta u_{t-1},\xi_{1:b})-F(x_{t-1}+\delta u_{t-1},\xi_{1:b}')  |^2\|u_t\|^2 \big)\nonumber
		\\ \overset{(i)}\leq & \frac{4(d+2)L_0^2}{\delta^2}\mathbb{E}\|x_t-x_{t-1}\|^2 + 8L_0^2\big((d+4)^2+(d+2)^2 \big) \nonumber
			\\&\quad \quad  \quad+\frac{2}{\delta^2 b^2} \mathbb{E}\big(|F(x_{t-1}+\delta u_{t-1},\xi_{1:b})-F(x_{t-1}+\delta u_{t-1},\xi_{1:b}')  |^2\|u_t\|^2 \big) \nonumber
			\\ \leq & \frac{4(d+2)L_0^2}{\delta^2}\mathbb{E}\|x_t-x_{t-1}\|^2 +\frac{4}{\delta^2b^2}\underbrace{\mathbb{E}|F(x_{t-1}+\delta u_{t-1},\xi_{1:b})- b f(x_{t-1}+\delta u_{t-1})|^2\|u_t\|^2}_{(P)} \nonumber
			\\&+ \frac{4}{\delta^2b^2}\underbrace{\mathbb{E}|F(x_{t-1}+\delta u_{t-1},\xi_{1:b}')- b f(x_{t-1}+\delta u_{t-1})|^2\|u_t\|^2}_{(Q)}+ 16L_0^2(d+4)^2,
	\end{align}
	where (i) follows from Lemma 1 in \cite{nesterov2017random} that $\mathbb{E}\|u\|^p\leq (d+p)^{p/2}$ for a $d$-dimensional standard Gaussian random vector. 
Our next step is to upper-bound $(P)$ and $(Q)$ in the above inequality. For $(P)$,	conditioning on $x_{t-1}$ and $u_{t-1}$ and noting that $\xi_{1:b}$ is independent of $u_t$, we have 
\begin{align}\label{p1}
& (P) = \mathbb{E}_{\xi_{1:b}}\Big| \sum_{\xi\in \xi_{1:b}}\big(F(x_{t-1}+\delta u_{t-1},\xi)-f(x_{t-1}+\delta u_{t-1})\big)\Big|^2\mathbb{E}_{u_t}\|u_t\|^2 \nonumber
\\ \leq & \; (d+2)\mathbb{E}_{\xi_{1:b}}\Big|  \sum_{\xi\in \xi_{1:b}}\big(F(x_{t-1}+\delta u_{t-1},\xi)-f(x_{t-1}+\delta u_{t-1})\big)\Big|^2 \nonumber
\\ = &\; b(d+2) \mathbb{E}_{\xi}|F(x_{t-1}+\delta u_{t-1},\xi)-f(x_{t-1}+\delta u_{t-1})|^2  + (d+2) \sum_{i\neq j,\xi_i,\xi_j\in \xi_{1:b}} \nonumber
\\&\langle \mathbb{E}_{\xi_i}F(x_{t-1}+\delta u_{t-1},\xi_i)-f(x_{t-1}+\delta u_{t-1}),\mathbb{E}_{\xi_j} F(x_{t-1}+\delta u_{t-1},\xi_j)-f(x_{t-1}+\delta u_{t-1})\rangle\nonumber
\\= & \; b(d+2) \mathbb{E}_\xi\|F(x_{t-1}+\delta u_{t-1},\xi)-f(x_{t-1}+\delta u_{t-1})\|^2 \leq  b(d+2)\sigma^2.
\end{align}
%where (i) follows from the fact that $\xi_i$ is independent of $\xi_j$ and $\mathbb{E}_{\}$
Unconditioning on $x_{t-1}$ and $u_{t-1}$ in the above equality yields $(P)\leq b(d+2)\sigma^2$. 
 For $Q$, we have 
 \begin{align}
 (Q) =& \; \mathbb{E}\big(|F(x_{t-1}+\delta u_{t-1},\xi_{1:b}')- b f(x_{t-1}+\delta u_{t-1})|^2\mathbb{E}_{u_t}\|u_t\|^2\, \big| x_{t-1},\xi_{1:b}',u_{t-1}\big) \nonumber
 \\ \leq &(d+2) \mathbb{E}|F(x_{t-1}+\delta u_{t-1},\xi_{1:b}')- b f(x_{t-1}+\delta u_{t-1})|^2,\nonumber
 \end{align}
 which, using an approach similar to the steps in~\eqref{p1}, yields
 \begin{align}\label{q1}
 (Q)\leq b(d+2)\sigma^2.
 \end{align}
 Combining~\eqref{pqo},~\eqref{p1} and~\eqref{q1} yields the proof when $F(x, \xi) \in C^{0,0}$.
 
 When function $F(x, \xi) \in C^{1,1}$, based on the definition of $\widetilde g_b(x_t)$, we have 
 \begin{align*}
 & \|\widetilde g_b(x_t)\|^2 = \frac{1}{\delta^2 b^2}|F(x_t+\delta u_t, \xi_{1:b}) -F(x_{t-1}+\delta u_{t-1},\xi_{1:b}) & \nonumber \\
 & \quad \quad \quad \quad \quad \quad \quad \quad \quad +F(x_{t-1}+\delta u_{t-1},\xi_{1:b})-F(x_{t-1}+\delta u_{t-1},\xi_{1:b}')  |^2 \|u_t\|^2 & \nonumber
 \\ & \leq \frac{2}{\delta^2 b^2} |F(x_t+\delta u_t,\xi_{1:b}) -F(x_{t-1}+\delta u_{t-1},\xi_{1:b})|^2 \|u_t\|^2 & \nonumber \\
 & \quad \quad \quad \quad \quad \quad \quad \quad \quad + \frac{2}{\delta^2 b^2} |F(x_{t-1}+\delta u_{t-1},\xi_{1:b})-F(x_{t-1}+\delta u_{t-1},\xi_{1:b}')  |^2 \|u_t\|^2, \nonumber
 \end{align*}
 which, taking expectation and using an approach similar to~\eqref{pqo}, yields 
 \begin{align}\label{opiis}
 \mathbb{E} \|\widetilde g(x_t)\|^2 \leq \frac{2}{\delta^2 b^2} \underbrace{\mathbb{E}|F(x_t+\delta u_t,\xi_{1:b}) -F(x_{t-1}+\delta u_{t-1},\xi_{1:b})|^2 \|u_t\|^2}_{(P)}+ \frac{8(d+2)\sigma^2}{\delta^2 b}. 
 \end{align}
 Our next step is to upper-bound $(P)$ in the above inequality. We first divide $(P)$ into the following three parts. 
 \begin{align}
 & (P) \leq 3\mathbb{E}\Big[ \underbrace{|F(x_t + \delta u_t, \xi_{1:b}) -F(x_t, \xi_{1:b}) - \inner{\delta u_t}{\nabla F(x_t,\xi_{1:b})} + \inner{\delta u_t}{\nabla F(x_t,\xi_{1:b})}|^2\|u_t\|^2}_{(P_1)} \nonumber\\
 & + \underbrace{|F(x_t,\xi_{1:b}) - F(x_{t-1},\xi_{1:b})|^2\|u_t\|^2}_{(P_2)}\nonumber\\
 & + \underbrace{|F(x_{t-1},\xi_{1:b}) - F(x_{t-1} + \delta u_{t-1},\xi_{1:b}) + \inner{\delta u_{t-1}}{\nabla F(x_{t-1},\xi_{1:b})} -\inner{\delta u_{t-1}}{\nabla F(x_{t-1},\xi_{1:b})}|^2\|u_t\|^2}_{(P_3)} \Big]. \label{eq: kaiyi}
 \end{align}
 Using the assumption that $F(x;\xi)\in C^{0,0}\cap C^{1,1}$, we have
 \begin{align}
 P_1 & \le b^2 L^2_1\delta^4\|u_t\|^6 + 2\delta^2| \inner{u_t}{\nabla F(x_t,\xi_{1:b})} |^2\|u_t\|^2, \nonumber\\
 P_2 &\le b^2 L_0^2  \|x_{t} - x_{t-1}\|^2\|u_t\|^2, \nonumber\\ 
 P_3 &\le b^2 L^2_1\delta^4\|u_{t-1}\|^4\|u_t\|^2  +2\delta^2 | \inner{u_{t-1}}{\nabla F(x_{t-1},\xi_{1:b})}|^2\|u_t\|^2. \nonumber
 \end{align}
 Plugging the above inequalities into~\eqref{eq: kaiyi}, we have
 \begin{align}\label{fanren}
 (P) \leq &3 b^2 L^2_1\delta^4\mathbb{E}\|u_t\|^6 + 6\delta^2\mathbb{E}| \inner{u_t}{\nabla F(x_t,\xi_{1:b})} |^2\|u_t\|^2 + 3 b^2 L_0^2\mathbb{E} \|x_t-x_{t-1}\|^2\|u_t\|^2 \nonumber
 \\ &+ 3 b^2 L^2_1\delta^4\mathbb{E}\|u_{t-1}\|^4\|u_t\|^2  +6\delta^2 \mathbb{E}| \inner{u_{t-1}}{\nabla F(x_{t-1},\xi_{1:b})}|^2\|u_t\|^2, 
 \end{align}
 Based on the results in~\cite{nesterov2017random}, we have  $\mathbb{E}_u[\|u\|^p]\le (d+p)^{p/2}$, $ \mathbb{E}[\inner{u_t}{\nabla F(x_t,\xi_{1:b})}^2\|u_t\|^2] \le (d+4) \|\nabla F(x_t,\xi_{1:b})\|^2$, $\mathbb{E}[\inner{u_{t-1}}{\nabla F(x_{t-1},\xi_{1:b})}^2] \le \|\nabla F(x_t,\xi_{1:b})\|^2$, which, in conjunction with \eqref{fanren}, yields
 \begin{align}\label{ggsimida}
 & (P)\leq 6 b^2 L^2_1\delta^4(d+6)^3  + 3 b^2 (d+2) L_0^2\mathbb{E} \|x_t-x_{t-1}\|^2 \nonumber
 \\ & \quad \quad \quad \quad  +6(d+4)\delta^2\mathbb{E}\|\nabla F(x_t,\xi_{1:b}) \|^2+6(d+2)\delta^2 \mathbb{E}\|\nabla F(x_{t-1},\xi_{1:b})\|^2 \nonumber
 \\ & \overset{(i)}\leq 6 b^2 L^2_1\delta^4(d+6)^3  + 3 b^2 (d+2) L_0^2\mathbb{E} \|x_t-x_{t-1}\|^2 +12 b^2 (d+4)\delta^2\mathbb{E}\|\nabla f(x_t) \|^2 \nonumber
 \\ & \quad \quad \quad +12 b (d+4)\delta^2\sigma_g^2 +12 b^2 (d+2)\delta^2 \mathbb{E}\|\nabla f(x_{t-1})\|^2 + 12 b (d+2)\delta^2\sigma_g^2 \nonumber
 \\  & \leq 6 b^2 L^2_1\delta^4(d+6)^3  + 3 b^2 (d+2) L_0^2\mathbb{E} \|x_t-x_{t-1}\|^2 \nonumber
 \\ & \quad \quad \quad +12 b^2 (d+4)\delta^2\mathbb{E}\|\nabla f(x_t) \|^2+12 b^2 (d+2)\delta^2 \mathbb{E}\|\nabla f(x_{t-1})\|^2 + 24 b (d+4)\delta^2\sigma_g^2.  
 \end{align}
 Combining~\eqref{ggsimida} and \eqref{opiis} yields
 \begin{align}
 \mathbb{E} \|\widetilde g_b(x_t)\|^2 \leq &12L^2_1\delta^2(d+6)^3  + \frac{6 (d+2) L_0^2\eta^2}{\delta^2}\mathbb{E} \|\widetilde g_b(x_{t-1})\|^2 \nonumber
 \\ &  +24(d+4)\mathbb{E}(\|\nabla f(x_t) \|^2+ \|\nabla f(x_{t-1})\|^2) + \frac{48(d+4)\sigma_g^2}{b}+ \frac{8(d+2)\sigma^2}{\delta^2 b},
 \end{align}
 which finishes the proof. 
\end{proof}

First, we analyze the convergence when the problem is non-smooth. 
%Lemma~\ref{le:variance11} shows that the estimation variance can be reduced if 
Based on Lemma~\ref{le:variance11}, we provide an upper bound on $\mathbb{E}\|x_{t+1}-x_t\|^2$.
\begin{lem}\label{le:online_ind}
Suppose Assumptions~\ref{asmp:BoundedVariance} and \ref{asmp:BoundedLipschitz} are satisfied. Then, we have 
\begin{align}
\mathbb{E}\|x_{t+1}-x_t\|^2 \leq \beta_1^t\Big( \mathbb{E}\|x_{1}-x_{0}\|^2 -\frac{\beta_2}{1-\beta_1}\Big)+\frac{\beta_2}{1-\beta_1},
\end{align}
where $\beta_1 =\frac{4\eta^2(d+2)L_0^2}{\delta^2} $ and $\beta_2 = 16\eta ^2 L_0^2(d+4)^2  +\frac{8\eta^2(d+2)\sigma^2}{\delta^2 b}$. 
\end{lem}
\begin{proof}
Based on the update that $x_{t+1}-x_t=-\eta \widetilde g_b(x_t)$ and Lemma~\ref{le:variance11}, we have 
\begin{align*}
\mathbb{E}\|x_{t+1}-x_t\|^2 =&\eta^2 \|\widetilde g_b(x_t)\|^2 \leq \eta^2 \Big( \frac{4(d+2)L_0^2}{\delta^2}\mathbb{E}\|x_t-x_{t-1}\|^2 + 16L_0^2(d+4)^2  + \frac{8(d+2)\sigma^2}{\delta^2 b}  \Big) \nonumber
\\ =&\frac{4\eta^2(d+2)L_0^2}{\delta^2} \mathbb{E}\|x_t-x_{t-1}\|^2 +16\eta ^2 L_0^2(d+4)^2  +\frac{8\eta^2(d+2)\sigma^2}{\delta^2 b} .
\\ = & \beta_1 \mathbb{E}\|x_t-x_{t-1}\|^2+\beta_2.
\end{align*}
Then, telescoping the above inequality yields the proof. 
%\begin{align*}
%\mathbb{E}\|x_{t+1}-x_t\|^2 \leq \beta_1^t\Big( \mathbb{E}\|x_{1}-x_{0}\|^2 -\frac{\beta_2}{1-\beta_1}\Big).
%\end{align*}
%Telescoping the above inequality over $t$ from $1$ to
\end{proof}
\subsection*{Nonsmooth Nonconvex Geometry}
Based on the above lemmas, we next provide the  convergence and complexity analysis for our proposed algorithm for the case where $F(x;\xi)$ is nonconvex and belongs to $C^{0,0}$. 
\begin{thm}
Suppose Assumptions~\ref{asmp:BoundedVariance} and \ref{asmp:BoundedLipschitz} are satisfied. Choose $\eta= \frac{\epsilon_f^{1/2}}{2(d+2)^{3/2}T^{1/2}L^2_0}, \delta = \frac{\epsilon_f}{(d+2)^{1/2}L_0}$ and $b=\frac{\sigma^2}{\epsilon_f^2}\geq 1$ for certain $\epsilon_f<1$.  Then, we have 
%\begin{align}
$\mathbb{E}\|\nabla f_\delta(x_\zeta)\|^2
%\leq  \mathcal{O}\left( \Big(1+\frac{\sigma^2}{\theta^{2}b}\Big)\frac{d^{3/2}}{\theta^{1/2}\sqrt{k}} \right) 
\leq \mathcal{O}\left( \frac{d^{3/2}}{\epsilon_f^{1/2}\sqrt{T}} \right) $ with the approximation error $|f_\delta (x_\zeta)-f(x_\zeta)|<\theta$, where $\zeta$ is uniformly sampled from $\{0, 1, \dots, T-1 \}$. 
%\end{align}
Then, to achieve an $\epsilon$-accurate stationary point of  $f_\delta$, the corresponding total function query complexity is given by 
\begin{align}
Tb =  \mathcal{O}\left( \frac{\sigma^2 d^{3}}{\epsilon_f^{3}\epsilon^{2}} \right).
\end{align}
\end{thm} 
\begin{proof}
	Recall that $f_\delta(x)=\mathbb{E}_{u}f(x+\delta u)$ is a smoothed approximation of  $f(x)$, where $u\in\mathbb{R}^d$ is a standard Gaussian random vector. Based on Lemma 2 in~\cite{nesterov2017random},  we have $f_\delta \in C^{1,1}$ with gradient-Lipschitz constant $L_\delta$ satisfying $L_\delta\leq \frac{d^{1/2}}{\delta} L_0$, and thus 
% we have 	
%Using Equation (12) in~\cite{nesterov2017random}, the gradient $\nabla F_\delta(\cdot)$ is  $L_1$-Lipschitz, and we have
\begin{align*}
f_\delta(x_{t+1}) \leq & f_\delta(x_t) +\langle \nabla f_\delta(x_t), x_{t+1}-x_t\rangle +\frac{L_\delta}{2} \|x_{t+1}-x_t\|^2
\\ \leq & f_\delta(x_t) +\langle \nabla f_\delta(x_t), x_{t+1}-x_t\rangle +\frac{d^{1/2}L_0}{2\delta} \|x_{t+1}-x_t\|^2
\\ = & f_\delta(x_t) -\eta \langle \nabla f_\delta(x_t), \widetilde g(x_t)\rangle + \frac{d^{1/2}L_0}{2\delta} \|x_{t+1}-x_t\|^2.
\end{align*}
Taking expectation over the above inequality and using $\mathbb{E}(\widetilde g(x_t) | x_t)=\nabla f_\delta(x_t)$, we have
\begin{align*}
\mathbb{E} f_\delta (x_{t+1}) \leq \mathbb{E} f_\delta (x_t) -\eta \mathbb{E}\|\nabla f_\delta(x_t)\|^2 + \frac{d^{1/2}L_0}{2\delta} \mathbb{E}\|x_{t+1}-x_t\|^2,
\end{align*}
which, in conjunction with Lemma~\ref{le:online_ind}, yields
\begin{align}
\mathbb{E} f_\delta (x_{t+1}) \leq \mathbb{E} f_\delta (x_t) -\eta \mathbb{E}\|\nabla f_\delta(x_t)\|^2 + \frac{d^{1/2}L_0}{2\delta} \beta_1^t\Big( \mathbb{E}\|x_{1}-x_{0}\|^2 -\frac{\beta_2}{1-\beta_1}\Big)+\frac{d^{1/2}L_0}{2\delta} \frac{\beta_2}{1-\beta_1}.
\end{align}
Telescoping the above inequality over $t$ from $0$ to $T-1$ yields
\begin{align*}
& \sum_{t=0}^{T-1}\eta \mathbb{E}\|\nabla f_\delta (x_t)\|^2 & \nonumber \\
& \leq f_\delta(x_0)- \inf_x f_\delta(x) + \frac{d^{1/2}L_0 T}{2\delta} \frac{\beta_2}{1-\beta_1} + \frac{d^{1/2}L_0}{2\delta} \Big( \mathbb{E}\|x_{1}-x_{0}\|^2 -\frac{\beta_2}{1-\beta_1}\Big)\sum_{t=0}^{T-1}\beta_1^t
\\ & = f_\delta(x_0)- \inf_x f_\delta(x) + \frac{d^{1/2}L_0 T}{2\delta} \frac{\beta_2}{1-\beta_1} + \frac{d^{1/2}L_0}{2\delta} \Big( \mathbb{E}\|x_{1}-x_{0}\|^2 -\frac{\beta_2}{1-\beta_1}\Big)\frac{1-\beta_1^T}{1-\beta_1}
\\ & \leq  f(x_0)- \inf_x f(x) + 2 \delta L_0 d^{1/2}+ \frac{d^{1/2}L_0 T}{2\delta} \frac{\beta_2}{1-\beta_1} + \frac{d^{1/2}L_0}{2\delta} \Big( \mathbb{E}\|x_{1}-x_{0}\|^2 -\frac{\beta_2}{1-\beta_1}\Big)\frac{1-\beta_1^T}{1-\beta_1},
\end{align*}
where the last inequality follows from Equation (3.11) in~\cite{ghadimi2013stochastic} and Equation (18) in~\cite{nesterov2017random}. Choose $\eta= \frac{\epsilon_f^{1/2}}{2(d+2)^{3/2}T^{1/2}L^2_0}$ and $\delta = \frac{\epsilon_f}{(d+2)^{1/2}L_0}$ with certain $\epsilon_f<1$, and set $T>\frac{1}{2\epsilon_f d}$. 
Then, we have $\beta_1 = \frac{1}{\epsilon_f(d+2)T}<\frac{1}{2}$, 
%Let us choose $\beta_1 = \frac{\delta^r}{2}< \frac{1}{2}$ for some $0<\delta<1$ and $r>0$, which implies that  $\eta^2 = \frac{\delta^{r+2}}{8(d+2)L_0^2}$. 
and thus the above inequality yields 
%Recalling that $\eta=\frac{1}{(d+2)\sqrt{k}}$, $\delta^2=\frac{8L_0^2}{(d+2)^2\sqrt{k}}$ and $k\geq (d+2)^2$, we have $\beta_1=\frac{4\eta^2(d+2)L_0^2}{\delta^2} =\frac{d+2}{2\sqrt{k}}\leq \frac{1}{2}$, which, in conjunction with the above inequality yields 
\begin{align}
\sum_{t=0}^{T-1}\eta \mathbb{E}\|\nabla f_\delta (x_t)\|^2 \leq &f(x_0)- \inf_x f(x) + 2 \delta L_0 d^{1/2}+ \frac{\beta_2 d^{1/2}L_0 T}{\delta} + \frac{d^{1/2}L_0\eta^2}{\delta}\mathbb{E}\|\widetilde g_b(x_0)\|^2.
\end{align}
Choosing $\zeta$  from $0,1,...,T-1$ uniformly at random, and rearranging  the above inequality, we have
\begin{align}
\mathbb{E}\|\nabla f_\delta(x_\zeta)\|^2 \leq & \; \frac{f(x_0)- \inf_x f(x)  }{\eta T} +\frac{2 \delta L_0 d^{1/2} }{\eta T} + \frac{d^{1/2}L_0\eta}{\delta T}\mathbb{E}\|\widetilde g(x_0)\|^2 \nonumber \\
& \quad \quad \quad + \frac{16\eta (d+4)^2d^{1/2}L_0^3 }{\delta}    +   \frac{ 8\eta (d+2)d^{1/2}L_0 \sigma^2}{\delta^3 b} & \nonumber \\
\leq & \mathcal{O}\left( \frac{1}{\eta T} + \frac{\delta L_0 d^{1/2}}{\eta T} +   \frac{d^{1/2}L_0\eta}{\delta T} + \frac{\eta d^{5/2}L_0^3 }{\delta}    +   \frac{ \eta d^{3/2}L_0 \sigma^2}{\delta^3 b}\right),
%\\ &+\frac{ d^{1/2}L_0 }{\delta}(16\eta  L_0^2(d+4)^2  +\frac{8\eta (d+2)\sigma^2}{\delta^2 b})\nonumber
%\\ =&  \frac{(d+2)(F(x_0)- \inf_x F(x)+L_1 \mathbb{E}\|x_{1}-x_{0}\|^2)}{\sqrt{k}} + \frac{8L_0^2L_1}{k}+ \frac{16(d+4)^2L_0^2L_1^2}{(d+2)\sqrt{k}}+\frac{(d+2)^2L_1\sigma^2}{L_0^2 b}\nonumber
\end{align}
which, in conjunction with $\eta= \frac{\epsilon_f^{1/2}}{2(d+2)^{3/2}T^{1/2}L^2_0}, \delta = \frac{\epsilon_f}{(d+2)^{1/2}L_0}$ and $b=\frac{\sigma^2}{\epsilon_f^2}$, yields
\begin{align}
\mathbb{E}\|\nabla f_\delta(x_\zeta)\|^2 \leq & \mathcal{O}\left( \frac{1}{\eta T} + \frac{\delta L_0 d^{1/2}}{\eta T } +   \frac{d^{1/2}L_0\eta}{\delta T} + \frac{\eta d^{5/2}L_0^3 }{\delta}    +   \frac{ \eta d^{3/2}L_0 \sigma^2}{\delta^3 b}\right) \nonumber
\\ \leq & \mathcal{O} \left(  \frac{d^{3/2}L^2_0}{\epsilon_f^{1/2}\sqrt{T}} + \frac{\epsilon_f^{1/2}d^{3/2}L_0^2}{\sqrt{T}} + \frac{1}{\epsilon_f^{1/2}d^{1/2}T^{3/2}} + \frac{d^{3/2}\sigma^2}{\epsilon_f^{5/2}\sqrt{T} b}\right) & \nonumber \\
\leq & \mathcal{O}\left( \Big(1+\frac{\sigma^2}{\epsilon_f^{2}b}\Big)\frac{d^{3/2}}{\epsilon_f^{1/2}\sqrt{T}} \right) \leq \mathcal{O}\left( \frac{d^{3/2}}{\epsilon_f^{1/2}\sqrt{T}} \right). \nonumber
\end{align}
Based on $ \delta = \frac{\epsilon_f}{(d+2)^{1/2}L_0}$ and Equation (18) in~\cite{nesterov2017random}, we have $|f_\delta(x)-f(x)| < \epsilon_f$. Then, to achieve an $\epsilon$-accurate stationary point of the smoothed function $f_\delta$ with approximation error $|f_\delta(x)-f(x)| <\epsilon_f, \epsilon_f<1$ , we need 
$T\leq \mathcal{O}(\epsilon_f^{-1}d^{3}\epsilon^{-2})$, and thus the corresponding total function query complexity is given by 
\begin{align}
Tb =  \mathcal{O}\left( \frac{\sigma^2 d^{3}}{\epsilon_f^{3}\epsilon^{2}} \right).
\end{align}
Then, the proof is complete. 
%According to Lemma 4 in~\cite{nesterov2017random}, we have $\|\nabla F_\delta(x_\zeta)\|^2 \geq \frac{1}{2}\|\nabla F(x_\zeta)\|^2-\frac{\delta^2}{4}L_1^2(d+6)^3$, which, in conjunction with the above inequality, yields
%\begin{align}
%\mathbb{E}\|\nabla F(x_\zeta)\|^2 \leq &  \frac{2(d+2)(F(x_0)- \inf_x F(x)+L_1 \mathbb{E}\|x_{1}-x_{0}\|^2)}{\sqrt{k}} + \frac{16L_0^2L_1}{k}+ \frac{32(d+4)^2L_0^2L_1^2}{(d+2)\sqrt{k}} \nonumber
%\\&+\frac{4L_1^2L_0^2(d+6)^3}{(d+2)^2\sqrt{k}}+\frac{2(d+2)^2L_1\sigma^2}{L_0^2 b}  \nonumber
%\\ \leq & \mathcal{O}\Big(\frac{d}{\sqrt{k}}+\frac{d^2\sigma^2}{b}\Big).
%\end{align}
%If we treat $L_0,L_1$
	\end{proof}
\subsection*{Nonsmooth Convex Geometry}
In this part, we provide the convergence and complexity  analysis for our proposed algorithm for the case where $F(x;\xi)$ is convex and belongs to $C^{0,0}$. 
\begin{thm}
Suppose Assumptions~\ref{asmp:BoundedVariance} and \ref{asmp:BoundedLipschitz} are satisfied and $\mathbb{E}\|\widetilde g_b(x_{0})\|^2\leq M d^2 T$ for certain constant $M>0$. Choose $\eta =\frac{1}{(d+2)\sqrt{T}L_0}$, $\delta = \frac{(d+2)^{1/2}}{\sqrt{T}}$, $b=\frac{\sigma^2 T}{d^2}$, and $T>d^2$.  Then, we have 
%\begin{align}
$\mathbb{E}\big(f(x_\zeta) - \inf_x f(x) \big) 
%\leq  \mathcal{O}\left( \Big(1+\frac{\sigma^2}{\theta^{2}b}\Big)\frac{d^{3/2}}{\theta^{1/2}\sqrt{k}} \right) 
\leq  \mathcal{O}\big(\frac{d}{\sqrt{T}}\big) $.
%\end{align}
Then, to achieve an $\epsilon$-accurate solution of  $f(x)$, the corresponding total function query complexity is given by 
\begin{align}
Tb = \mathcal{O} \Big( \frac{\sigma^2 d^2}{\epsilon^{4}}\Big).
\end{align}
	\end{thm}
\begin{proof}
	Let $x^*$ be a  minimizer of the function $f$, i.e. $x^*=\arg\min_x f(x)$. Then, we have 
\begin{align*}
\|x_{t+1} - x^*\|^2 &= \|x_t - \eta \widetilde{g}_b(x_t) -x^*\|^2 \nonumber\\
&= \|x_{t} - x^*\|^2 -2\eta \inner{\widetilde{g}_b(x_t)}{x_t - x^*} + \mathbb{E}\|x_{t+1}-x_{t}\|^2.
\end{align*}
Telescoping the above inequality over $t$ from $0$ to $T-1$ yields that
\begin{align*}
\|x_T - x^*\|^2 = \|x_0 - x^*\|^2 - 2\eta \sum_{t=0}^{T-1} \inner{\widetilde{g}_b(x_t)}{x_t - x^*} +  \sum_{t=0}^{T-1} \mathbb{E}\|x_{t+1}-x_{t}\|^2. 
\end{align*}
Taking expectation in the above equality using the fact that $\mathbb{E}[\widetilde{g}_b(x_t)|x_t] = \nabla f_\delta(x_t)$, we further obtain that
\begin{align}\label{eq: wocaca}
& \mathbb{E}\|x_T - x^*\|^2 = \|x_0 - x^*\|^2 - 2\eta \sum_{t=0}^{T-1} \mathbb{E}\inner{\nabla f_\delta(x_t)}{x_t - x^*} +  \sum_{t=0}^{T-1} \mathbb{E}\|x_{t+1}-x_{t}\|^2 \nonumber\\
&\overset{(i)}{\le} \|x_0 - x^*\|^2 - 2\eta \sum_{t=0}^{T-1} \mathbb{E}\big(f_\delta(x_t) - f_\delta(x^*) \big) + \sum_{t=0}^{T-1} \mathbb{E}\|x_{t+1}-x_{t}\|^2 \nonumber\\
%&\le \|x_0 - x^*\|^2 - 2\eta \sum_{t=0}^{k-1} \mathbb{E}\big(F_n(x_t) - F_n(x^*) \big) +2\eta\sum_{t=0}^{k-1} \mathbb{E}\Big(|F_n^\delta(x_t)-F_n(x_t)|+|F_n^\delta(x^*)-F_n(x^*)|\Big)\nonumber\\
%&\quad+ \eta^2 \sum_{t=0}^{k-1} \mathbb{E}\|\widetilde{g}(x_t)\|^2 \nonumber\\
&\overset{(ii)}{\le} \|x_0 - x^*\|^2 - 2\eta \sum_{t=0}^{T-1} \mathbb{E}\big(f(x_t) - f(x^*) \big) +4\eta\delta L_0 \sqrt{d}T+ \sum_{t=0}^{T-1} \mathbb{E}\|x_{t+1}-x_{t}\|^2, 
\end{align} 
where (i) follows from the convexity of $f_\delta$ and (ii) uses the fact that $|f_\delta(x) - f(x)|\le \delta L_0 \sqrt{d}$. Then,  rearranging the above inequality yields
\begin{align*}
& \frac{1}{T}\sum_{t=0}^{T-1}\mathbb{E}\big(f(x_t) - f(x^*) \big) \leq \frac{\|x_0-x^*\|^2}{\eta T}+ 4\delta L_0 \sqrt{d} + \frac{1}{\eta T} \sum_{t=0}^{T-1}\mathbb{E}\|x_{t+1}-x_{t}\|^2 \nonumber
\\& \overset{(i)}\leq \frac{\|x_0-x^*\|^2}{\eta T}+ 4\delta L_0 \sqrt{d} + \frac{1}{\eta T} \sum_{t=0}^{T-1} \Big( \beta_1^t\Big( \mathbb{E}\|x_{1}-x_{0}\|^2 -\frac{\beta_2}{1-\beta_1}\Big)+\frac{\beta_2}{1-\beta_1}\Big) \nonumber
\\ & \leq \frac{\|x_0-x^*\|^2}{\eta T}+ 4\delta L_0 \sqrt{d} + \frac{1}{\eta T} \frac{1-\beta_1^T}{1-\beta_1} \Big(\mathbb{E}\|x_{1}-x_{0}\|^2 -\frac{\beta_2}{1-\beta_1}\Big)+\frac{\beta_2}{\eta(1-\beta_1)},
\end{align*} 
where (i) follows from Lemma~\ref{le:online_ind} with $\beta_1 =\frac{4\eta^2(d+2)L_0^2}{\delta^2} $ and $\beta_2 = 16\eta ^2 L_0^2(d+4)^2  +\frac{8\eta^2(d+2)\sigma^2}{\delta^2 b}$. Recalling $\eta =\frac{1}{(d+2)\sqrt{T}L_0}$, $\delta = \frac{(d+2)^{1/2}}{\sqrt{T}}$, $b=\frac{\sigma^2 T}{d^2}$, and $T>d^2$, we have $\beta_1 < 1/2$, and the above inequality yields
\begin{align*}
\frac{1}{T}\sum_{t=0}^{T-1}\mathbb{E}\big(f(x_t) - f(x^*) \big)  \leq & \frac{\|x_0-x^*\|^2}{\eta T}+ 4\delta L_0 \sqrt{d} + \frac{2\eta}{T} \mathbb{E}\|\widetilde g_b(x_{0})\|^2+32\eta  L_0^2(d+4)^2  \nonumber
\\  & \quad \quad \quad \quad \quad \quad +\frac{16\eta(d+2)\sigma^2}{\delta^2 b} \leq\mathcal{O}\left( \frac{d}{\sqrt{T}}+ \frac{ \mathbb{E}\|\widetilde g_b(x_{0})\|^2}{dT^{3/2}}\right), 
\end{align*}
which, combined with $\mathbb{E}\|\widetilde g_b(x_{0})\|^2\leq M d^2 T$ for constant $M$ and choosing $\zeta$ from $0,..,T-1$ uniformly at random, yields 
\begin{align}
\mathbb{E}\big(f(x_\zeta) - f(x^*) \big)  \leq  \mathcal{O}\Big(\frac{d}{\sqrt{T}}\Big).
\end{align}
To achieve an $\epsilon$-accurate solution, i.e., $\mathbb{E}\big(f(x_\zeta) - f(x^*) \big) <\epsilon$, we need $T=\mathcal{O}(d^2\epsilon^{-2})$, and hence the corresponding function query complexity is given by 
\begin{align}
Tb\leq \mathcal{O} \Big( \sigma^2 d^2\epsilon^{-4}\Big),
\end{align}
which finishes the proof. 
	\end{proof}

\subsection{Analysis  in Smooth Setting} 	

In this section, we  provide the convergence and complexity analysis for the proposed gradient estimator when function $F(x, \xi) \in C^{1,1}$

\subsection*{Smooth Nonconvex Geometry}
In this part, we provide the  convergence and complexity analysis for the proposed gradient estimator  for the case where $F(x;\xi)$ is nonconvex and belongs to $C^{0,0}\cap C^{1,1}$. 
\begin{thm}
Suppose Assumptions~\ref{asmp:BoundedVariance}, \ref{asmp:BoundedLipschitz} and \ref{asmp:BoundedVariance_Gradient} are satisfied and $\mathbb{E}\|\widetilde g_b(x_0)\|^2 \leq M T d^{8/3}$ for certain constant $M>0$. Choose $\eta = \frac{1}{4(d+2)^{4/3}\sqrt{T}\max(L_0,L_1)}< \frac{1}{8L_1}, \delta = \frac{1}{(d+2)^{5/6} T^{1/4}}$ and $ b=\max\big(\sigma^2,\frac{\sigma_g^2}{\sqrt{T}d^{5/3}}\big)\sqrt{T}$.  Then, we have 
%\begin{align}
$\mathbb{E}\|\nabla f_\delta(x_\zeta)\|^2
%\leq  \mathcal{O}\left( \Big(1+\frac{\sigma^2}{\theta^{2}b}\Big)\frac{d^{3/2}}{\theta^{1/2}\sqrt{k}} \right) 
\leq \mathcal{O}\Big( \frac{d^{4/3}}{\sqrt{T}}\Big)$.
Then, to achieve an $\epsilon$-accurate stationary point of  $f$, the  total function query complexity is given by 
\begin{align}
Tb =  \mathcal{O}\big(\sigma^2d^4\epsilon^{-3}+\sigma_g^2d\epsilon^{-2}\big).
\end{align}
\end{thm} 
\begin{proof}
Based on Equation (12) in~\cite{nesterov2017random}, the smoothed function $f_\delta\in C^{1,1}$ with gradient-Lipschitz constant less than $L_1$. Then, we have 
\begin{align*}
f_\delta(x_{t+1}) \leq & f_\delta(x_t) +\langle \nabla f_\delta(x_t), x_{t+1}-x_t\rangle +\frac{L_1}{2} \|x_{t+1}-x_t\|^2
\\ = & f_\delta(x_t) -\eta \langle \nabla f_\delta(x_t), \widetilde g_b(x_t)\rangle +\frac{L_1}{2}\|x_{t+1}-x_t\|^2.
\end{align*}
Let $\alpha= \frac{6 (d+2) L_0^2\eta^2}{\delta^2}$, $\beta=12L^2_1\delta^2(d+6)^3  + \frac{48(d+4)\sigma_g^2}{b}+ \frac{8(d+2)\sigma^2}{\delta^2 b}$ and $p_{t-1}=24(d+4)\mathbb{E}(\|\nabla f(x_t) \|^2+ \|\nabla f(x_{t-1})\|^2)$. Then, telescoping the bound in Lemma~\ref{le:variance11} in the smooth case yields
\begin{align}\label{ggsmoiis}
\mathbb{E} \|\widetilde g_b(x_t)\|^2  & \leq \alpha^t \mathbb{E}\|\widetilde g_b(x_0)\|^2  +   \sum_{j=0}^{t-1}\alpha^{t-1-j}p_j + \beta\sum_{j=0}^{t-1}\alpha^j & \nonumber \\
& \leq \alpha^t \mathbb{E}\|\widetilde g_b(x_0)\|^2  +   \sum_{j=0}^{t-1}\alpha^{t-1-j}p_j + \frac{\beta(1-\alpha^t)}{1-\alpha}.
\end{align}
%To simplify notations, let $p_{}$
Taking expectation over the above inequality and using $\mathbb{E}(\widetilde g_b(x_t) | x_t)=\nabla f_\delta(x_t)$, we have
\begin{align*}
\mathbb{E} f_\delta (x_{t+1}) \leq \mathbb{E} f_\delta (x_t) -\eta \mathbb{E}\|\nabla f_\delta(x_t)\|^2 + \frac{L_1\eta^2}{2} \mathbb{E}\|\widetilde g_b(x_t)\|^2.
\end{align*}
Telescoping the above inequality over $t$ from $0$ to $T-1$ yields
\begin{align}
& \mathbb{E} f_\delta (x_{k}) \leq f_\delta (x_0) -\eta \sum_{t=0}^{T-1}\mathbb{E}\|\nabla f_\delta(x_t)\|^2 + \frac{L_1\eta^2}{2} \sum_{t=0}^{T-1} \mathbb{E}\|\widetilde g_b(x_t)\|^2\nonumber
\\ & \overset{(i)}\leq f_\delta (x_0) -\eta \sum_{t=0}^{T-1}\mathbb{E}\|\nabla f_\delta(x_t)\|^2 + \frac{L_1\eta^2}{2}\mathbb{E}\|\widetilde g_b(x_0)\|^2 & \nonumber \\
& \quad \quad \quad +\frac{L_1\eta^2}{2} \sum_{t=1}^{T-1} \left( \alpha^t \mathbb{E}\|\widetilde g_b(x_0)\|^2  +   \sum_{j=0}^{t-1}\alpha^{t-1-j}p_j + \frac{\beta(1-\alpha^t)}{1-\alpha}   \right)\nonumber
\\& = f_\delta (x_0) -\eta \sum_{t=0}^{T-1}\mathbb{E}\|\nabla f_\delta(x_t)\|^2 + \frac{1-\alpha^T}{1-\alpha}\frac{L_1\eta^2}{2}\mathbb{E}\|\widetilde g_b(x_0)\|^2  & \nonumber \\
& \quad \quad \quad +\frac{L_1\eta^2}{2} \sum_{j=0}^{T-2}\sum_{t=0}^{T-2-j}\alpha^{t}p_j +\frac{L_1\eta^2}{2} \sum_{t=1}^{T-1}\frac{\beta(1-\alpha^t)}{1-\alpha}  \nonumber
\end{align}
Since $\sum_{j=0}^{T-2}\sum_{t=0}^{T-2-j}\alpha^{t}p_j \leq \sum_{j=0}^{T-2}\sum_{t=0}^{T-2}\alpha^{t}p_j $, we have that
\begin{align}
&  \mathbb{E} f_\delta (x_{k}) \leq f_\delta (x_0) -\eta \sum_{t=0}^{T-1}\mathbb{E}\|\nabla f_\delta(x_t)\|^2 + \frac{1-\alpha^T}{1-\alpha}\frac{L_1\eta^2}{2}\mathbb{E}\|\widetilde g_b(x_0)\|^2 \nonumber \\
& \quad \quad \quad \quad \quad +\frac{L_1\eta^2}{2} \sum_{j=0}^{T-2}\sum_{t=0}^{T-2}\alpha^{t}p_j +\frac{L_1\eta^2}{2} \sum_{t=1}^{T-1}\frac{\beta(1-\alpha^t)}{1-\alpha} & \nonumber
\\ & \leq f_\delta (x_0) -\eta \sum_{t=0}^{T-1}\mathbb{E}\|\nabla f_\delta(x_t)\|^2 + \frac{1-\alpha^T}{1-\alpha}\frac{L_1\eta^2}{2}\mathbb{E}\|\widetilde g_b(x_0)\|^2 & \nonumber \\
& \quad \quad \quad +\frac{L_1\eta^2}{2} \frac{1-\alpha^{T-1}}{1-\alpha}\sum_{t=0}^{T-2}p_t +\frac{L_1\eta^2}{2} \sum_{t=1}^{T-1}\frac{\beta(1-\alpha^t)}{1-\alpha} \nonumber
\end{align}
where (i) follows from~\eqref{ggsmoiis}. Choose $\eta = \frac{1}{4(d+2)^{4/3}\sqrt{T}\max(L_0,L_1)}$ and $\delta = \frac{1}{(d+2)^{5/6} T^{1/4}}$. Then, we have $\alpha\leq \frac{3}{8}<\frac{1}{2}$, and the above inequality yields
\begin{align}
\mathbb{E} f_\delta (x_{k})  \leq f_\delta (x_0) -\eta \sum_{t=0}^{k-1}\mathbb{E}\|\nabla f_\delta(x_t)\|^2 + L_1\eta^2\mathbb{E}\|\widetilde g_b(x_0)\|^2 +L_1\eta^2\sum_{t=0}^{T-2}p_t +L_1\eta^2 T\beta. \nonumber
\end{align}
Rearranging the above inequality and using $|f_\delta(x) - f|\leq \frac{\delta^2}{2}L_1d$ and $\|\nabla f_\delta(x)-\nabla f(x)\|\leq \frac{\delta}{2} L_1 (d+3)^{3/2}$ proved in~\cite{nesterov2017random}, we have 
\begin{align}
\mathbb{E} & f(x_{k})  \leq f (x_0) +\delta^2 L_1 d-\frac{\eta}{2} \sum_{t=0}^{T-1}\mathbb{E}\|\nabla f(x_t)\|^2 +\frac{\eta T}{4}\delta^2 L_1^2 (d+3)^3 & \nonumber \\
& \quad \quad \quad \quad + L_1\eta^2\mathbb{E}\|\widetilde g_b(x_0)\|^2 +L_1\eta^2\sum_{t=0}^{T-2}p_t +L_1\eta^2 T \beta \nonumber
\\ \leq & f(x_0) +\delta^2 L_1 d-\frac{\eta}{2} \sum_{t=0}^{T-1}\mathbb{E}\|\nabla f(x_t)\|^2 +\frac{\eta T}{4}\delta^2 L_1^2 (d+3)^3 & \nonumber \\
& \quad \quad \quad \quad  + L_1\eta^2\mathbb{E}\|\widetilde g_b(x_0)\|^2 +2L_1\eta^2 \sum_{t=0}^{T-1} \|\nabla f(x_t)\|^2+L_1\eta^2 T \beta. \nonumber
\end{align}
Choosing $\zeta$ from $0,...,T-1$ uniformly at random, we obtain from the above inequality that 
\begin{align*}
\big(  \frac{1}{2} - 2L_1\eta\big) \mathbb{E} \|\nabla f(x_\zeta)\|^2 \leq & \frac{f(x_0)-\inf_x f(x)}{\eta T} + \frac{\delta^2 L_1 d}{\eta T} \nonumber \\
& \quad \quad \quad \quad \quad +\frac{L_1^2}{4}\delta^2 (d+3)^3 +\frac{L_1\eta\mathbb{E}\|\widetilde g_b(x_0)\|^2}{T} + L_1 \eta \beta, 
\end{align*}
which, in conjunction with $\eta = \frac{1}{4(d+2)^{4/3}\sqrt{T}\max(L_0,L_1)}< \frac{1}{8L_1}, \delta = \frac{1}{(d+2)^{5/6}T^{1/4}}, \beta=12L^2_1\delta^2(d+6)^3  + \frac{48(d+4)\sigma_g^2}{b}+ \frac{8(d+2)\sigma^2}{\delta^2 b}, b=\max\big(\sigma^2,\frac{\sigma_g^2}{\sqrt{T}d^{5/3}}\big)\sqrt{T}$ and $\mathbb{E}\|\widetilde g_b(x_0)\|^2 \leq M T d^{8/3}$, yields 
\begin{align*}
\mathbb{E} \|\nabla f(x_\zeta)\|^2 \leq \mathcal{O}\Big( \frac{d^{4/3}}{\sqrt{T}}+ \frac{d^{2/3}}{T}+ \frac{d^{4/3}}{\sqrt{T}}+ \frac{d^{4/3}}{\sqrt{T}}+\frac{1}{T}+\frac{\sigma_g^2}{d^{1/3}b\sqrt{T}}+\frac{d^{4/3}\sigma^2}{b} \Big) \leq \mathcal{O}\Big( \frac{d^{4/3}}{\sqrt{T}}\Big).
\end{align*}
Then, to achieve an $\epsilon$-accurate stationary point of  function $f$, i.e., $\mathbb{E}\|\nabla f(x_\zeta)\|^2<\epsilon$, we need $T =\mathcal{O}(d^{8/3}\epsilon^{-2})$the total number of function query is given by $Tb\leq \mathcal{O}\big(\sigma^2d^4\epsilon^{-3}+\sigma_g^2d\epsilon^{-2}\big)$.
\end{proof}
	
\subsection*{Smooth Convex Geometry}
In this part, we provide the  convergence and complexity analysis for the proposed gradient estimator  for the case where $F(x;\xi)$ is convex and belongs to $C^{0,0}\cap C^{1,1}$. 
\begin{thm}
Suppose Assumptions~\ref{asmp:BoundedVariance}, \ref{asmp:BoundedLipschitz} and \ref{asmp:BoundedVariance_Gradient} are satisfied and $\mathbb{E}\|\widetilde g_b(x_0)\|^2 \leq M T d^{2}$ for certain constant $M>0$. Choose $\eta = \frac{1}{192(d+2)\sqrt{T}\max(L_0,L_1)}$ and $\delta^2 =\frac{1}{\sqrt{T}}$ and $b=\max\big(\frac{\sigma_g^2}{\sqrt{T}},\sigma^2\big)\sqrt{T}/d$.  Then, we have 
%\begin{align}
$\mathbb{E}\|\nabla f_\delta(x_\zeta)\|^2
%\leq  \mathcal{O}\left( \Big(1+\frac{\sigma^2}{\theta^{2}b}\Big)\frac{d^{3/2}}{\theta^{1/2}\sqrt{k}} \right) 
\leq \mathcal{O} \Big( \frac{d}{\sqrt{T}}+ \frac{d^2}{T}\Big)$.
Then, to achieve an $\epsilon$-accurate stationary point of  $f$, the  total function query complexity is given by 
\begin{align}
Tb =  \mathcal{O}\big(\sigma^2d^2\epsilon^{-3}+\sigma_g^2d\epsilon^{-2}\big).
\end{align}
\end{thm} 
\begin{proof}
Using an approach similar to \eqref{eq: wocaca}, we have 
\begin{align*}
\mathbb{E}\|x_T - x^*\|^2 &
%= \|x_0 - x^*\|^2 - 2\eta \sum_{t=0}^{k-1} \mathbb{E}\inner{\nabla F_\delta(x_t)}{x_t - x^*} +  \sum_{t=0}^{k-1} \mathbb{E}\|x_{t+1}-x_{t}\|^2 \nonumber\\
%&{\le} \|x_0 - x^*\|^2 - 2\eta \sum_{t=0}^{k-1} \mathbb{E}\big(F_\delta(x_t) - F_\delta(x^*) \big) + \sum_{t=0}^{k-1} \mathbb{E}\|x_{t+1}-x_{t}\|^2 \nonumber\\
%&\le \|x_0 - x^*\|^2 - 2\eta \sum_{t=0}^{k-1} \mathbb{E}\big(F_n(x_t) - F_n(x^*) \big) +2\eta\sum_{t=0}^{k-1} \mathbb{E}\Big(|F_n^\delta(x_t)-F_n(x_t)|+|F_n^\delta(x^*)-F_n(x^*)|\Big)\nonumber\\
%&\quad+ \eta^2 \sum_{t=0}^{k-1} \mathbb{E}\|\widetilde{g}(x_t)\|^2 \nonumber\\
{\le} \|x_0 - x^*\|^2 - 2\eta \sum_{t=0}^{T-1} \mathbb{E}\big(f(x_t) - f(x^*) \big) +2\eta\delta^2 L_1 d T+ \sum_{t=0}^{T-1}\eta^2 \mathbb{E}\|\widetilde g_b(x_{t})\|^2, 
\end{align*}
where the last inequality follows from Equation (19) in~\cite{nesterov2017random}. 
Let $\alpha= \frac{6 (d+2) L_0^2\eta^2}{\delta^2}$, $\beta=12L^2_1\delta^2(d+6)^3  + \frac{48(d+4)\sigma_g^2}{b}+ \frac{8(d+2)\sigma^2}{\delta^2 b}$ and $p_{t-1}=24(d+4)\mathbb{E}(\|\nabla f(x_t) \|^2+ \|\nabla f(x_{t-1})\|^2)$. Then, 
%telescoping the bound in Lemma~\ref{le:varismooth} yields
%\begin{align}\label{ggsmoiis}
%\mathbb{E} \|\widetilde g(x_t)\|^2  \leq \alpha^t \mathbb{E}\|\widetilde g(x_0)\|^2  +   \sum_{j=0}^{t-1}\alpha^{t-1-j}p_j + \beta\sum_{j=0}^{t-1}\alpha^j\leq \alpha^t \mathbb{E}\|\widetilde g(x_0)\|^2  +   \sum_{j=0}^{t-1}\alpha^{t-1-j}p_j + \frac{\beta(1-\alpha^t)}{1-\alpha}.
%\end{align}
combining the above inequality with \eqref{ggsmoiis} yields
\begin{align}
& \mathbb{E}\|x_T - x^*\|^2  \leq \|x_0 - x^*\|^2 - 2\eta \sum_{t=0}^{T-1} \mathbb{E}\big(f(x_t) - f(x^*) \big) +2\eta\delta^2 L_1 d T + \eta^2 \mathbb{E} \|\widetilde g_b(x_0)\|^2 \nonumber
\\& \quad \quad \quad \quad \quad \quad \quad + \sum_{t=1}^{T-1}\eta^2\Big(\alpha^t \mathbb{E}\|\widetilde g_b(x_0)\|^2  +   \sum_{j=0}^{t-1}\alpha^{t-1-j}p_j + \frac{\beta(1-\alpha^t)}{1-\alpha} \Big) \nonumber
\\& \leq \|x_0 - x^*\|^2 - 2\eta \sum_{t=0}^{T-1} \mathbb{E}\big(f(x_t) - f(x^*) \big) +2\eta\delta^2 L_1 d T + \eta^2\frac{1-\alpha^T}{1-\alpha} \mathbb{E} \|\widetilde g_b(x_0)\|^2 \nonumber
\\& \quad \quad + \eta^2 \sum_{j=0}^{T-2}\sum_{t=0}^{T-2}\alpha^{t}p_j  + \eta^2 \sum_{t=1}^{T-1}\frac{\beta(1-\alpha^t)}{1-\alpha} \nonumber
\\& \leq \|x_0 - x^*\|^2 - 2\eta \sum_{t=0}^{T-1} \mathbb{E}\big(f(x_t) - f(x^*) \big) +2\eta\delta^2 L_1 d T + \eta^2\frac{1-\alpha^T}{1-\alpha} \mathbb{E} \|\widetilde g_b(x_0)\|^2 \nonumber
\\&\quad \quad  + 24(d+4)\eta^2 \frac{1-\alpha^{T-1}}{1-\alpha}\sum_{t=0}^{T-2}\mathbb{E}(\|\nabla f(x_{t+1}) \|^2+ \|\nabla f(x_{t})\|^2) + \eta^2 \sum_{t=1}^{T-1}\frac{\beta(1-\alpha^t)}{1-\alpha}.
\end{align}
Recalling $\eta = \frac{1}{192(d+2)\sqrt{T}\max(L_0,L_1)}$ and $\delta^2 =\frac{1}{\sqrt{T}}$, we have $\alpha<\frac{1}{2}$, and thus the above inequality yields
\begin{align}
\mathbb{E}\|x_T - x^*\|^2  \leq & \|x_0 - x^*\|^2 - 2\eta \sum_{t=0}^{T-1} \mathbb{E}\big(f(x_t) - f(x^*) \big) +2\eta\delta^2 L_1 d T + 2\eta^2\mathbb{E} \|\widetilde g_b(x_0)\|^2 \nonumber
\\&+ 48(d+4)\eta^2\sum_{t=0}^{T-2}\mathbb{E}(\|\nabla f(x_{t+1}) \|^2+ \|\nabla f(x_{t})\|^2) +2 T \eta^2 \beta.
\end{align}
Since the convexity implies that $\frac{1}{2L_1}\|\nabla f(x) \|^2\leq f(x)-f(x^*)$ for any $x$, rearranging the above inequality yields
\begin{align}
& (2-192(d+4)L_1\eta) \frac{1}{T}\sum_{t=0}^{T-1}\mathbb{E}(f(x_t)-f(x^*)) \nonumber \\
& \leq \frac{\|x_0-x^*\|^2}{\eta T}+ 2\delta^2 L_1 d + \frac{2\eta \mathbb{E}\|\widetilde g_b(x_0)\|^2}{T} +24\eta L^2_1\delta^2(d+6)^3 + \frac{96\eta (d+4)\sigma_g^2}{b}+ \frac{16\eta(d+2)\sigma^2}{\delta^2 b},
\end{align}
which, in conjunction with $\mathbb{E}\|\widetilde g_b(x_0)\|^2\leq M d^2 T$ for certain constant $M>0$, $b=\max\big(\frac{\sigma_g^2}{\sqrt{T}},\sigma^2\big)\sqrt{T}/d$ and recalling that  $\zeta$ is chosen from $0,...,T-1$ uniformly at random, yields
\begin{align}
\mathbb{E}(f(x_\zeta)-f(x^*)) \leq \mathcal{O} \Big( \frac{d}{\sqrt{T}}+ \frac{d^2}{T}\Big).
\end{align}
Then, to achieve an $\epsilon$-accurate solution, i.e.,  $\mathbb{E}(f(x_\zeta)-f(x^*))\leq \epsilon$, we need $T=\mathcal{O}(d^2\epsilon^{-2})$, and thus the corresponding query complexity is given by 
\begin{align}
Tb \leq \mathcal{O}(\sigma^2d^2\epsilon^{-3}+ \sigma_g^2d\epsilon^{-2})
\end{align}
\end{proof}

\input{Online_Proof}
